# Supplementary material for: Machine Learning Hamiltonians are Accurate Energy-Force Predictors
Source: arXiv:2602.16897 source file (2026-07-04)
Supplement: Supplementary file 1 [file 99_appendix_old.tex]

\appendix
\section{Additional Preliminary}

\subsection{Kohn-Sham density functional theory.}
\label{app:dft}
The density functional theory (DFT) is a cornerstone of quantum chemistry and materials science, offering a computationally tractable framework for approximating the electronic structure of many-body systems. As directly solving the many-electron Schrödinger equation~\cite{schrodinger1926undulatory} is prohibitively expensive for systems with many particles, DFT reformulates the problem by expressing ground-state properties as a functional of the electron density $\rho(\mathbf{r})$. Since $\rho(\mathbf{r})$ depends only on three spatial coordinates, this significantly reduces the computational complexity regardless of the number of electrons.

In practical applications, DFT is most commonly implemented via the Kohn–Sham formulation~\cite{hohenberg1964inhomogeneous, kohn1965self}, which introduces a system of non-interacting electrons that reproduces the true ground-state density of the interacting system. The KF-DFT for $N$-particle system uses the parameterization $\smash{\Psi(\mathbf{r}_{1},\ldots, \mathbf{r}_{N}) = \sum_{i=1}^{N}\psi_{i}(\mathbf{r}_{i})}$ using single-particle orbitals $\{\psi_{i}\}_{i=1}^{N}$ where  $\rho(\mathbf{r}) = \sum_{n=1}^{N}|\psi_{i}(\mathbf{r}_{i})|^{2}.$ The KS-equations are:
\begin{equation}
    \left[ -\frac{1}{2}\nabla^2 + V_{\text{ext}}(\mathbf{r}) + V_{\text{H}}[\rho](\mathbf{r}) + V_{\text{xc}}[\rho](\mathbf{r}) \right] \psi_i(\mathbf{r}) = \epsilon_i \psi_i(\mathbf{r}),
\end{equation}
where $\nabla^2$ is the Laplacian operator for kinetic energy, $V_{\text{ext}}$ is the external potential from the nuclei, $V_{\text{H}}$ is the Hartree potential, $V_{\text{xc}}$ is the exchange-correlation potential, and $\psi_i$, $\epsilon_i$ are the Kohn–Sham orbitals and their corresponding energies.

\subsection{Group theory}
\label{app:prelim}

We briefly introduce key concepts from group theory, providing the necessary background to understand the motivation behind equivariant designs in Hamiltonian prediction.

\textbf{Groups.}  
A \textit{group} $ G $ is a non-empty set equipped with a binary operation $ \circ: G \times G \to G $, satisfying the following axioms:

\begin{itemize}
    \item \textbf{Associativity}: For all $ a, b, c \in G $, $(a \circ b) \circ c = a \circ (b \circ c)$.
    \item \textbf{Identity}: There exists an identity element $ e \in G $ such that for all $ a \in G $, $ e \circ a = a \circ e = a $.
    \item \textbf{Inverse}: For each $ a \in G $, there exists an inverse $ a^{-1} \in G $ such that $ a \circ a^{-1} = a^{-1} \circ a = e $.
    \item \textbf{Closure}: For all $ a, b \in G $, the result $ a \circ b $ is also in $ G $.
\end{itemize}

We typically simplify notation by omitting $\circ$, writing $ ab $ instead of $ a \circ b $. Groups can be finite or infinite, discrete or continuous, compact or non-compact. Group theory~\cite{kosmann2010groups} provides a rigorous mathematical foundation for describing symmetries in physical systems~\cite{cornwell1997group}, an essential perspective for designing physically informed machine learning models.

\textbf{Group actions.}  
To make group theory applicable to structures in mathematics and physics, we define how groups act on sets. A group $ G $ is said to act on a set $ \mathcal{X} $ if there exists a function $ \cdot_\mathcal{X}: G \times \mathcal{X} \to \mathcal{X} $\footnote{The subscript of group action operator for indicating the input and output space is often omitted when clear from context, \textit{i.e.,} $g\cdot_\mathcal X h=g\cdot h$.} such that for all $ g, h \in G $ and $ x \in X $, the following conditions hold: (1) $ e \cdot_{\mathcal{X}} x = x $, where $ e $ is the identity element of $ G $, and (2) $ (gh) \cdot_{\mathcal{X}} x = g \cdot_{\mathcal{X}} (h \cdot_{\mathcal{X}} x) $. These conditions ensure that the group operation is compatible with its action on the set. In practice, such group actions often correspond to geometric transformations, such as translations, rotations, or reflections, on points or functions defined over Euclidean space.

\textbf{Equivariance.}  
When working with structured data such as molecular geometries or fields, it is often desirable that the operations we apply preserve the symmetries of the underlying space. A function $ f: \mathcal X \to \mathcal Y $ is said to be \textit{equivariant} with respect to group actions $ \cdot_{\mathcal X} $ on the input space $\mathcal{X}$ and $ \cdot_{\mathcal Y} $ on the output space $ \mathcal Y $, if it satisfies
\begin{equation}
    f(g\cdot_{\mathcal X} x) = g\cdot_{\mathcal Y} f(x), \quad \forall g \in G, x \in \mathcal X.
\end{equation}
 This means that applying a group transformation before or after the function yields consistent results. In physical systems, such as those governed by rotational symmetry (\textit{e.g.}, SO(3) in molecules), equivariance ensures that rotated inputs yield correspondingly rotated outputs. This property is critical in designing models that generalize well across symmetrically equivalent configurations.

\textbf{Group representations.}  
Group actions on vector spaces are formalized through the notion of representations. A \textit{representation} of a group $ G $ on a vector space $ V $ is a homomorphism $ \rho: G \to \operatorname{GL}(V) $, where $ \operatorname{GL}(V) $ denotes the group of invertible linear transformations on $ V $. This mapping associates each group element with a linear operator that describes how the group acts on the space. The vector space $ V $ is referred to as the \textit{representation space}, and its dimension defines the representation's size.

In finite-dimensional real spaces $ V = \mathbb{R}^d $, these representations are often expressed as invertible matrices $ \mathbf{D}(g) \in \mathbb{R}^{d \times d} $. For instance, the group SO(3) of 3D rotations is represented by orthogonal matrices $ \mathbf{g} \in \text{SO(3)}$ and its 3D rotation matrix $\mathbf{R}\in\mathbb{R}^{3 \times 3}$ acting on vectors $\mathbf{x} \in \mathbb{R}^3$ via matrix multiplication $\mathbf{D}(\mathbf{g})\mathbf{x} = \mathbf{R}\mathbf{x}$.

Two representations $ \mathbf{D}(g) $ and $ \mathbf{D}'(g) $ are said to be \textit{equivalent} if they are related by a change of basis:
\begin{equation}
\mathbf{D}'(g) = \mathbf{Q}^{-1} \mathbf{D}(g) \mathbf{Q},
\end{equation}
for some invertible matrix $ \mathbf{Q} $. Such equivalence indicates that the two representations describe the same group action under different coordinate systems.

\subsection{Irreducible representations}
\label{app:irreps}
\textbf{Irreducible representations (Irreps).}  
A representation $\rho: G \rightarrow \operatorname{GL}(V)$ of a group $G$ on a vector space $V$ is called \textit{irreducible} if it does not contain any nontrivial invariant subspace. More formally, a subspace $W \subseteq V$ is said to be invariant under the representation $\rho$ if for all group elements $g \in G$ and all vectors $w \in W$, the action satisfies:
\begin{equation}
\rho(g)w \in W.
\end{equation}
Then, the representation $\rho$ is irreducible if the only invariant subspaces it admits are the trivial subspace $\{0\}$ and the entire representation space $V$.

Irreducible representations play a fundamental role because any finite-dimensional unitary representation of a compact group can be uniquely decomposed into a direct sum of irreducible representations, up to isomorphism~\cite{wigner2012group}. This decomposition is foundational in analyzing the symmetry properties and constructing equivariant neural network architectures.



For the rotation group SO(3), the irreps are completely characterized by non-negative integers  $\ell \in \mathbb{N}_0$. Each irreducible representation $D^{(\ell)}: \text{SO(3)} \rightarrow \mathbb{C}^{(2\ell+1)\times(2\ell+1)}$ has dimension $2l + 1$ and is explicitly realized by the action on spherical harmonics $Y_m^l(\theta,\phi)$. For a function $ f: S^2 \rightarrow \mathbb{C} $ can be expanded in the basis of spherical harmonics as:
\begin{equation}
f(\theta, \phi) = \sum_{l=0}^{\infty}\sum_{m=-l}^{l} f_{lm} Y_m^l(\theta,\phi),
\end{equation}
where $f_{lm} \in \mathbb{C}$ is the complex coefficients of the spherical harmonics. The action of a rotation $\mathbf{R} \in \text{SO}(3)$ on $f$ is defined as:
\begin{equation}
(\mathbf{R} \cdot f)(\theta,\phi) = f(\mathbf{R}^{-1}\cdot(\theta,\phi)) = \sum_{l=0}^{\infty}\sum_{m=-\ell}^{\ell}\sum_{m'=-\ell}^{\ell} D_{mm'}^{(\ell)}(\mathbf R)\, f_{\ell m'} Y_m^{\ell}(\theta,\phi),
\end{equation}
where $D^{(\ell)}(\mathbf{R})$ is the Wigner D-matrix corresponding to the irreducible representation labeled by $\ell$, acting linearly on the vector of expansion coefficients $\mathbf{f}^{(\ell)} = (f_{-\ell}, f_{-\ell+1}, \dots, f_{\ell}) \in \mathbb{C}^{(2\ell+1)}$. Explicitly, under rotation:
\begin{equation}
\mathbf{f}^{(\ell)} \xrightarrow{\mathbf{R}} D^{(\ell)}(\mathbf{R})\mathbf{f}^{(\ell)}.
\end{equation}

Thus, irreps serve as the fundamental building blocks in constructing functions and features that transform equivariantly under the action of SO(3).

\textbf{Clebsch–Gordan tensor product.}
Given two irreps $D^{(\ell_1)}$, $D^{(\ell_2)}$ of SO(3), their tensor product $D^{(\ell_1)}\otimes D^{(\ell_2)}$ acts on the tensor product space and is generally reducible. It decomposes into a direct sum of irreps:
\begin{equation}
D^{(\ell_1)}\otimes_{\text{CG}} D^{(\ell_2)} \cong \bigoplus_{\ell=|\ell_1-\ell_2|}^{\ell_1+\ell_2} D^{(\ell)},
\end{equation}
where the decomposition is governed by Clebsch–Gordan (CG) coefficients. CG coefficients enable a basis transformation from the product space to irreps, playing crucial roles in quantum angular momentum coupling and equivariant neural networks.

Explicitly, for vectors $\mathbf{u}^{(\ell_1)}\in \mathbb{C}^{(2l_1+1)}$ and $\mathbf{v}^{(\ell_2)}\in \mathbb{C}^{(2\ell_2+1)}$, their CG tensor product produces an irreducible feature $\mathbf{w}^{(\ell)}\in\mathbb{C}^{(2\ell+1)}$:
\begin{equation}
    w^{(\ell)}_m = \sum_{m_1,m_2} C_{(\ell_1,m_1),(\ell_2,m_2)}^{(\ell,m)}u^{(\ell_1)}_{m_1}v^{(\ell_2)}_{m_2}.
\end{equation}
This construction ensures that $\mathbf{w}^{(\ell)}$ transforms correctly under $\mathbf{R}\in \text{SO(3)}$:
\begin{equation}
    \left(D^{(\ell_1)}(\mathbf{R})\mathbf{u}^{(\ell_1)}\right)
    \otimes_{\text{CG}}\left(D^{(\ell_2)}
    (\mathbf{R})\mathbf{v}^{(\ell_2)}\right)= D^{(\ell)}(\mathbf{R})\mathbf{w}^{(\ell)}.
\end{equation}
Thus, CG tensor products ensure equivariant transformations, fundamental to maintaining consistency and symmetry in equivariant neural architectures.


\textbf{Tensor field networks (TFN).}
The TFN~\cite{thomas2018tensor} is a widely used architecture that achieves SE(3)-equivariance by explicitly encoding features as irreps of SO(3) and using spherical harmonics to process directional information. Each feature vector at a node is decomposed into spherical tensor components $\boldsymbol{V}^{(\ell)}\in \mathbb C^{(2\ell+1)}$, where $\ell$ denotes the order of the irreducible representation. The key component of the TFN layer is equivariant convolution and self-interaction. For the equivariant convolution, the filter function is generated by the spherical harmonic functions $Y^\ell_m({\hat{\mathbf r}_{ij}})$ are applied to the direction between atoms $i$ and $j$, \textit{i.e.}, $\hat {\mathbf{r}}_{ij}=(\mathbf{r}_i-\mathbf{r}_j)/\|\mathbf{r}_i-\mathbf{r}_j\|$, and are modulated by a learnable radial function $R(\|\mathbf{r}_{ij}\|)$, implemented as an MLP to produce the filter:
\begin{equation}
    F^{(\ell_{\text{in}},\ell_f)}(\mathbf r_{ij})=R^{(\ell_{\text{in}},\ell_f)}(\|\mathbf{r}_{ij}\|)Y^{\ell_f}_m(\hat {\mathbf{r}}_{ij}).
\end{equation}
The equivariant convolution aggregates information from neighboring nodes set $\mathcal N$ using the tensor product between the filters and neighboring features:
\begin{equation}
    \tilde{V}^{(\ell_{\text{out}})}_i=\sum_{j \in \mathcal{N}}\left(F^{(\ell_{\text{in}},\ell_f)}_c(\mathbf r_{ij}) \otimes V^{(\ell_{\text{in}})}_j\right)^{(\ell_{\text{out}})},
\end{equation}
where $\ell_\text{out} \in \{|\ell_{\text{in}}-\ell_f|,\ldots,(\ell_\text{in}+\ell_f)\}$. This convolution ensures that the result transforms equivariantly under rotation.

The self-interaction step applies a linear transformation over the channel dimension to each irreps independently:
\begin{equation}
    \tilde{V}^{(\ell)}_{icm}=\sum_{c'}w_{cc'}V^{(\ell)}_{ic'm},
\end{equation}
preserving equivariance due to the linearity and diagonal structure in the irrep indices. By construction, all operations in TFNs are equivariant to SE(3), allowing them to model tensorial and directional quantities while respecting physical symmetries. This makes them especially well-suited for applications in molecular modeling, quantum chemistry, and materials science, where equivariance is crucial for generalization and physical accuracy.

\subsection{Symmetry and equivariance of RH-DFT}
\label{app:KS-DFT-sym}
\textbf{Spherical harmonics and atomic orbital basis.}
To numerically solve the Kohn–Sham equations, electronic wavefunctions are typically expanded in a basis of atomic orbitals. These orbitals are constructed using spherical harmonics $Y^\ell_m(\theta, \phi)$, which form a complete orthonormal basis on the sphere $\mathbb{S}^2$ and transform under the irreducible representations $D^{(\ell)}$ of the rotation group $\text{SO(3)}$. An atomic orbital basis function takes the form~\cite{koch2015chemist}:
\begin{equation}
    \phi_{n\ell m}(\mathbf{r}) = R_{n\ell}(\|\mathbf{r}\|) Y^\ell_m(\theta, \phi),
\end{equation}
where $R_{n\ell}(\|\mathbf{r}\|)$ is a radial function (e.g., Gaussian~\cite{gill1994molecular} or Slater-type~\cite{slater1930atomic,hehre1969self}), and $Y^\ell_m$ captures the angular component. Here, $n$ is the principal quantum number, $\ell$ is the orbital angular momentum quantum number, and $m\in\{-\ell,\dots,\ell\}$ is the magnetic quantum number~\cite{griffiths2018introduction}.

These basis functions are central to Kohn–Sham DFT calculations, as molecular orbitals are expressed as linear combinations of atomic orbitals:
\begin{equation}
    \psi_i(\mathbf{r}) = \sum_{\alpha = (n\ell m)} C_{\alpha i} \, \phi_{n\ell m}(\mathbf{r} - \mathbf{r}_\alpha),
\end{equation}
where $\mathbf{C} \in \mathbb{R}^{B \times O}$ is the orbital coefficient matrix, $B$ is the number of basis functions, and $O$ is the number of occupied orbitals.

\textbf{Block Hamiltonian matrix.}
\label{app:full_hamiltonian}
The Hamiltonian matrix in RH-DFT can be decomposed according to the angular momentum quantum numbers $\ell$ grouping associated with the atomic orbitals. Specifically, let $\mathbf{H}^{(\ell,\ell')}\in \mathbb{C}^{(2\ell+1)\times(2\ell'+1)}$ denote the submatrix representing the coupling between two angular momentum numbers $\ell$ and $\ell'$. Under a rotation $\mathbf{R} \in \text{SO(3)}$, each such sub-matrix $\mathbf{H}^{(\ell,\ell')}$ transforms equivariantly according to the SO(3) irreps as follows:
\begin{equation}
\mathbf{H}^{(\ell,\ell')}[\mathcal{D}(\mathbf{R})\mathbf{C}] = D^{(\ell)}(\mathbf{R})\bigl(\mathbf{H}^{(\ell,\ell')}[\mathbf{C}]\bigr)D^{(\ell')}(\mathbf{R})^{-1},
\label{eq:block_hamiltonian}
\end{equation}
where atomic orbitals are grouped by their $\ell$ and $\ell'$, $\mathcal{D\mathbf{(R)}}$ is block diagonal Wigner-D matrix, and $D^\ell$ and $D^{\ell'}$ are Wigner D-matrices for $\ell$ and $\ell'$, respectively. These submatrices $\mathbf{H}^{(\ell,\ell')}$, called orbital-wise Hamiltonian blocks, are the minimal building blocks of the full Hamiltonian that respect SO(3)-equivariance and have $(2\ell+1)\times(2\ell'+1)$ elements which corresponds to the combination of the magnetic quantum number $m$ and $m'$.

\textbf{Full Hamiltonian matrix.}
\label{app:full_hamiltonian}
In practice, basis functions are grouped not only by their angular momentum, but also by the atom they are centered on. For atom $i$, we denote its angular momentum support as $L_i = \{\ell_1, \ell_2, \ldots\}$, where each $\ell_k$ corresponds to its atomic shell (\textit{e.g.}, $s$, $p$, $d$) represented in the basis set. 

From this atomic partitioning, the Hamiltonian can be reorganized into block form where each submatrix $\mathbf{H}_{ij}^{(\ell,\ell')}$ corresponds to the interaction between angular momentum $\ell \in L_i$ of atom $i$ and $\ell' \in L_j$ of atom $j$. The full Hamiltonian $\mathbf{H}$ is thus a structured matrix composed of $K \times K$ blocks, where $K = \sum_i |L_i|$ is the total number of irreps (angular momentum groups) across all atoms, where $|L_i|$ denotes the cardinality of the set.

To construct the full Hamiltonian matrix, we first form the atom-pair matrix $\mathbf{H}_{ij}$ for every atom-pair $(i,j)$. This atom-pair matrix gathers all interactions between the angular momentum orbital groupings on the two atoms:
\begin{equation}
    \label{eq:atomwise_ham}
    \mathbf{H}_{ij} = 
    \begin{bmatrix}
    \mathbf{H}_{ij}^{(\ell_0,\ell_0')} & \mathbf{H}_{ij}^{(\ell_0,\ell_1')} & \cdots \\
    \mathbf{H}_{ij}^{(\ell_1,\ell_0')} & \mathbf{H}_{ij}^{(\ell_1,\ell_1')} & \cdots \\
    \vdots & \vdots & \ddots
    \end{bmatrix},\qquad \ell_k \in L_i, \quad \ell'_k \in L_j,
\end{equation}
where $\mathbf{H}_{ij}^{(\ell,\ell')}\in \mathbb{C}^{(2\ell +1)\times(2\ell'+1)}$ denotes the interaction between angular momentum $\ell \in L_i$ of atom $i$ and $\ell' \in L_j$ of atom $j$.

Next, we place these atom-pair blocks into a global block matrix to obtain the full RH Hamiltonian matrix:
The full Hamiltonian matrix $\mathbf{H} \in \mathbb{C}^{n \times n}$, where $n = \sum_{\ell} (2\ell+1)$, is assembled by concatenating the atom-pair blocks:
\begin{equation}
    \mathbf{H} = 
    \begin{bmatrix}
    \mathbf{H}_{ii} & \mathbf{H}_{ji} & \cdots \\
    \mathbf{H}_{ij} & \mathbf{H}_{jj} & \cdots \\
    \vdots & \vdots & \ddots
    \end{bmatrix},\quad n = \sum_{i \in \mathcal{M}}\sum_{\ell\in {L_i}} (2\ell+1),
\end{equation}
for every atom-pair $(i,j)$ in the molecule $\mathcal{M}$.

For better intuition, we illustrate a schematic structure of the Hamiltonian matrix in \cref{fig:hamiltonian_structure-sub-1}. Here, blocks corresponding to $s$, $p$, and $d$ orbitals are arranged according to their angular momentum, highlighting the blockwise symmetry pattern induced by the underlying spherical harmonics basis.


\begin{figure}[t]
    \centering
    \includegraphics[width=\textwidth]{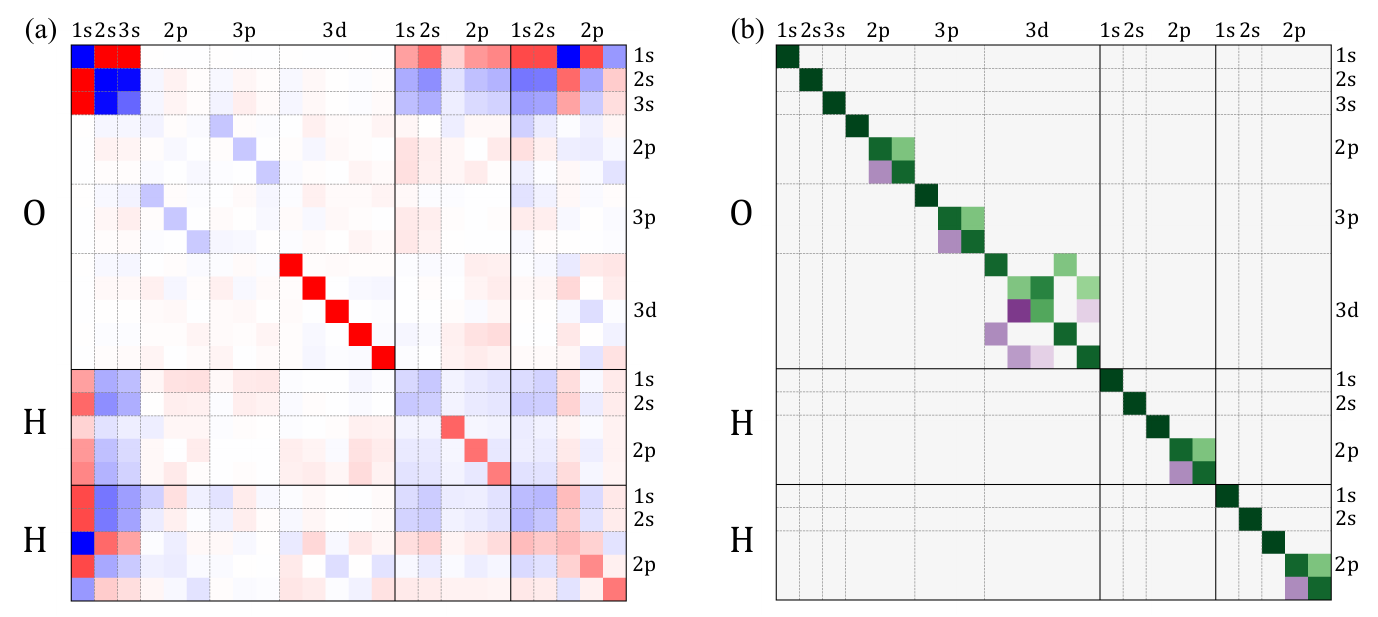}    {\phantomsubcaption\label{fig:hamiltonian_structure-sub-1}%
     \phantomsubcaption\label{fig:hamiltonian_structure-sub-2}}%
    \caption{(a) Schematic illustration of the full Hamiltonian matrix $\mathbf{H}$ for a water molecule (\ce{H2O}). Color intensity indicates the magnitude of matrix elements, with red representing larger values and blue representing smaller values. (b) Schematic illustration of the full Wigner D-matrix $\mathcal{D}$ corresponding to $\mathbf{H}$, where green denotes larger values and purple denotes smaller values. Gray solid and dashed lines separate molecular blocks and orbital blocks, respectively, corresponding to submatrices defined by atomic orbital pairs.}
    \label{fig:hamiltonian_structure}
\end{figure}

\textbf{Rotational equivariance of full Hamiltonian.}
The global action of a rotation $\mathbf{R}$ on the basis is encoded by the block-diagonal matrix as follows \cref{eq:block_diagnoal_D}:
\begin{equation}
    \mathcal{D}(\mathbf{R}) =  D^{(\ell_{1})}(\mathbf{R}) \oplus \cdots \oplus D^{(\ell_{K})}(\mathbf{R})=\begin{bmatrix}
        D^{(\ell_1)}(\mathbf{R}) & 0  & \cdots &  \\
        0 & D^{(\ell_2)}(\mathbf{R}) & \cdots &  \\
    \vdots & \vdots & \ddots
        
    \end{bmatrix},
\end{equation}
where each block $D^{\ell}(\mathbf{R})$ corresponds to the Wigner D-matrix for angular momentum $l$. The Hamiltonian matrix as a whole then transforms under rotation as:
\begin{equation}
    \mathbf{H}[\mathbf{C}] \xrightarrow{\mathbf{R}} \mathbf{H}[\mathbf{R} \cdot \mathbf{C}] = \mathbf{R} \cdot\mathbf{H}[\mathbf{C}]= \mathcal{D}(\mathbf{R}) \, \mathbf{H}[\mathbf{C}] \, \mathcal{D}(\mathbf{R})^{-1}.
\end{equation}

This global equivariance condition guarantees that the Hamiltonian transforms consistently with molecular rotations, preserving the physical structure of the system. Leveraging this symmetry is critical for constructing SE(3)-equivariant machine learning models, which not only respect physical laws but also improve model generalization and interpretability in quantum chemistry tasks. For better intuition, we illustrate a schematic structure of the Wigner D-matrix in \cref{fig:hamiltonian_structure-sub-2}.


\clearpage

\section{Training and sampling algorithms, and fine-tuning objective}

\subsection{Training and sampling algorithms}
\label{app:algorithms}

We investigate two types of prior distributions for the initial Hamiltonian $\mathbf{H}_0$: Gaussian orthogonal ensemble (GOE) and tensor expansion-based (TE) priors. For the GOE prior, we sample each matrix entry independently as $M_{ij} \sim \mathcal{N}(0, \sigma^2)$, where we set $\sigma^2=1.0$ for MD17 and $\sigma^2 = 0.1$ for QH9. 

For TE prior, we sample each irreducible component $\mathbf{w}^{l}$ by drawing its radial norm from $\operatorname{LogNormal}(1, \sigma^2=0.1)$ and applying a uniform SO(3) rotation to construct the full equivariant basis, which is then mapped to the Hamiltonian space via tensor expansion.

These choices provide flexibility in modeling different types of initial distributions, depending on the target dataset and symmetry constraints. Formal definitions and proofs of equivariance for both priors are provided in \cref{app:proof_GOE} and \cref{app:proof_tensor_expansion_multi}.

The training and sampling procedures based on the above rotationally invariant priors are summarized in \cref{algo:train} and \cref{algo:sample}, respectively.

\begin{algorithm}[H]
\caption{QHFlow training procedure}
\label{algo:train}
\begin{algorithmic}[1]
\REQUIRE Dataset of molecular configurations $\{\mathcal{M}_i\}$, target Hamiltonians $\mathbf{H}_{1,\mathcal{M}}$, overlap matrix $\mathbf{S}_{\mathcal{M}}$, model $f_\theta$
\FOR{each training step}
    \STATE Sample minibatch $\mathcal{B} = \{\mathcal{M}_i\}_{i=1}^B$
    \FOR{each $\mathcal{M}_i$ in $\mathcal{B}$}
        \STATE Sample initial Hamiltonian $\mathbf{H}_{0}\sim p_0$ and time $t \sim \mathcal{U}(0, 1)$
        \STATE Compute interpolated Hamiltonian: $\mathbf{H}_{t,\mathcal{M}} = (1 - t)\mathbf{H}_{0} + t\mathbf{H}_{1,\mathcal{M}}$
        \STATE Predict $\mathbf{H}_{1,\mathcal{M}}^{(\theta)} = f_\theta(\mathbf{H}_{t,\mathcal{M}}, \mathbf{S}_{\mathcal{M}}, \mathcal{M}, t)$
        \STATE Compute flow matching loss: $\mathcal{L}_i =  \|\mathbf{H}_{1,\mathcal{M}}^{(\theta)} - \mathbf{H}_{1,\mathcal{M}}\|^2$
    \ENDFOR
    \STATE Compute $\mathcal{L} = \frac{1}{B} \sum_{i=1}^B \mathcal{L}_i$, update $\theta \leftarrow \theta - \eta \nabla_\theta \mathcal{L}$
\ENDFOR
\end{algorithmic}
\end{algorithm}

\begin{algorithm}[H]
\caption{QHFlow sampling procedure}
\label{algo:sample}
\begin{algorithmic}[1]
\REQUIRE Molecular configuration $\mathcal{M}$, initial Hamiltonian $\mathbf{H}_0 \sim p_0$, model $f_\theta$, time discretization $\{t_0, t_1,\ldots, t_K\}$ where $t_0=0$ and $t_K=1$
\STATE Initialize $\mathbf{H}_{t_0} = \mathbf{H}_0$
\FOR{$k = 0$ to $K - 1$}
    \STATE Predict target Hamiltonian: $\smash{\mathbf{H}^{(\theta)}_{1,\mathcal{M}} \leftarrow f_\theta(\mathbf{H}_{t_k}, \mathbf{S}, \mathcal{M}, t_k)}$
    \STATE Compute conditional vector field: $v_{t_k, \theta} \leftarrow {(\mathbf{H}^{(\theta)}_{1,\mathcal{M}} - \mathbf{H}_{t_k})}/{(1 - t_k)}$
    \STATE Update Hamiltonian: $\mathbf{H}_{t_{k+1}} \leftarrow \mathbf{H}_{t_k} + (t_{k+1} - t_k) \cdot v_{t_k, \theta}$
\ENDFOR
\STATE Output $\hat{\mathbf{H}}_1 = \mathbf{H}_{t_K}$
\end{algorithmic}
\end{algorithm}


These algorithms ensure that training aligns the predicted vector field with the true conditional flow, while inference produces a final Hamiltonian via integration through the learned ODE trajectory. This design ensures SE(3)-equivariance and physical consistency throughout the training and prediction processes.


\subsection{Fine-tuning objective}
\label{app:finetune}

After pre-training with the flow matching objective, we further fine-tune QHFlow to enhance its spectral accuracy by introducing energy alignment objectives. To implement the energy alignment objective, we adopt the weighted alignment loss (WALoss) from WANet~\cite{lienhancing}.

\textbf{Property of the RH-equation.}  
The relationship between the Hamiltonian matrix $\mathbf{H}$, the coefficient matrix $\mathbf{C}$, and the orbital energy matrix $\boldsymbol{\epsilon}$ is governed by the Roothaan–Hall equation:
\begin{equation}
    \mathbf{H}\mathbf{C} = \mathbf{S}\mathbf{C}\boldsymbol{\epsilon},
\end{equation}
where $\mathbf{S}$ is overlap matrix. Using orthonormality condition $\mathbf{C}^\top \mathbf{S} \mathbf{C} = \mathbf{I}$, this relation simplifies to:
\begin{equation}
    \mathbf{C}^\top \mathbf{H} \mathbf{C} = \boldsymbol{\epsilon}.
\end{equation}
This identity forms the foundation for designing spectral alignment objectives.

\textbf{Weighted alignment loss (WALoss).}  
WALoss encourages the predicted Hamiltonian $\hat{\mathbf{H}}$ to match the spectral structure of the converged SCF Hamiltonian $\mathbf{H}^\star$. Let $\mathbf{C}^\star$ and $\boldsymbol{\epsilon}^\star$ denote the eigenvectors and eigenvalues of $\mathbf{H}^\star$, respectively. We define WALoss as:
\begin{equation}
\mathcal{L}_{\text{WALoss}} = \left\| \operatorname{diag}\left( (\mathbf{C}^\star)^\top \hat{\mathbf{H}} \mathbf{C}^\star \right) - \boldsymbol{\epsilon}^\star \right\|_2,
\end{equation}
where $\operatorname{diag}(\cdot)$ extracts the diagonal elements and $\|\cdot\|_2$ denotes the L2 norm.

To emphasize physically important states, we place larger weights on eigenvalues up to the Lowest unoccupied molecular orbital (LUMO) \textit{i.e.}, the $k+1$ lowest-energy orbitals. By projecting $\hat{\mathbf{H}}$ onto the fixed eigenbasis $\mathbf{C}^\star$, WALoss promotes alignment with the ground-truth spectrum. However, it is important to note that $(\mathbf{C}^\star)^\top \hat{\mathbf{H}} \mathbf{C}^\star$ does not exactly diagonalize $\hat{\mathbf{H}}$ unless $\hat{\mathbf{H}} = \mathbf{H}^\star$. Nevertheless, minimizing this discrepancy helps guide $\hat{\mathbf{H}}$ toward the correct eigenspectrum, improving orbital energy prediction and SCF behavior.

\textbf{Overall fine-tuning objective.}  
Our final finetuning objective combines the flow matching loss with WALoss:
\begin{equation}
\mathcal{L}_{\text{total}} = \mathcal{L}_{\text{CFM}} + \lambda_{\text{WA}} \mathcal{L}_{\text{WA}},
\end{equation}
where $\lambda_{\text{WA}}$ is the weighting coefficients controlling the contributions of the energy alignment terms, and we chose $\lambda_{\text{WA}}=2.0$ for the finetuning.

\clearpage
\section{Proofs and additional details}
\subsection{Proof of SE(3)-equivariance of GOE}
\label{app:proof_GOE}

Let $ \mathbf{M} \in \mathbb{R}^{n \times n} $ be a symmetric matrix drawn from the Gaussian orthogonal ensemble (GOE), characterized by:
\begin{equation}
    \mathbb{E}[M_{ij}] = 0, \quad \operatorname{Var}(M_{ij}) = \sigma^2, \quad \text{with } M_{ij} = M_{ji}, \text{ and independent entries for } i \leq j.
\end{equation}
Let $\mathbf{D} = \mathcal{D}(\mathbf{R})$ denote an orthogonal matrix representing a Wigner D-transformation corresponding to a rotation $ \mathbf{R} \in \mathrm{SO}(3) $, satisfying orthogonality \textit{i.e.} $ \mathbf{D} \mathbf{D}^\top = \mathbf{I} $. We define the rotated matrix as:
\begin{equation}
    \mathbf{M}' = \mathbf{DMD}^\top, \quad \text{with } M'_{ij} = \sum_{k, l} D_{ik} M_{kl} D_{jl}.
\end{equation}

We aim to show that the distribution of $ \mathbf{M}' $ is the same as that of $ \mathbf{M} $, i.e., that GOE is invariant under conjugation by orthogonal transformations:
\begin{equation}
\rho(\mathbf{M}) = \rho(\mathbf{DMD}^\top).
\end{equation}
To establish this, it suffices to verify that the first and second moments of the entries in $ \mathbf{M}' $ match those of GOE.

\textbf{Mean.}
Since $ \mathbb{E}[M_{kl}] = 0 $ for all $ k, l $, we have:
\begin{align}
    \mathbb{E}[M'_{ij}] = \sum_{k, l} D_{ik} D_{jl} \mathbb{E}[M_{kl}] = 0.
\end{align}

\textbf{Covariance.}
We now compute the covariance of the entries $ M'_{ab} $ and $ M'_{cd} $:
\begin{align}
    \mathbb{E}[M'_{ab} M'_{cd}]
    &= \mathbb{E}\left[ \left( \sum_{i, j} D_{ai} D_{bj} M_{ij} \right) \left( \sum_{k, l} D_{ck} D_{dl} M_{kl} \right) \right] \\
    &= \sum_{i,j,k,l} D_{ai} D_{bj} D_{ck} D_{dl} \, \mathbb{E}[M_{ij} M_{kl}].
\end{align}
Using the independence and zero mean of GOE entries, we know:
\begin{equation}
    \mathbb{E}[M_{ij} M_{kl}] = \sigma^2 \delta_{ik} \delta_{jl}.
\end{equation}
Thus,
\begin{align}
    \mathbb{E}[M'_{ab} M'_{cd}]
    &= \sigma^2 \sum_{i,j} D_{ai} D_{bj} D_{ci} D_{dj} \\
    &= \sigma^2 \left( \sum_i D_{ai} D_{ci} \right) \left( \sum_j D_{bj} D_{dj} \right) \nonumber\\
    &= \sigma^2 (\mathbf{D} \mathbf{D}^\top)_{ac} (\mathbf{D} \mathbf{D}^\top)_{bd} \nonumber\\
    &= \sigma^2 \delta_{ac} \delta_{bd}.
\end{align}

This matches the covariance structure of the original GOE matrix. Since both $ \mathbf{M} $ and $ \mathbf{M}' $ are jointly Gaussian with zero mean and identical covariances, we conclude:
\begin{equation}
\mathbf{DMD}^\top \sim \mathbf{M}, \quad \text{i.e., GOE is invariant under orthogonal conjugation.}
\end{equation}

This proves that the GOE prior is SO(3)-invariant, even for the high-rank Wigner D-matrices $\ell \ge 2$.


\subsection{Proof of the SE(3)-equivariance of tensor expansion operation}
\label{app:proof_tensor_expansion}

Since the $\mathbf{w}^{(\ell)}$ is the irrep vector, the $m$-th entry  $w^{\ell}_m$ transforms under rotation $\mathbf{R} \in \text{SO(3)}$ as:
\begin{equation}
    w^{(\ell)}_m \xrightarrow{\mathbf{R}} \left(\mathbf{R}\cdot\mathbf w^{(\ell)}\right)_m= \left(\sum_{m'} D^{(\ell)}_{mm'}(\mathbf{R})\, w^{(\ell)}_{m'}\right),
    \label{eq:app_te_transform}
\end{equation}
where $D^{(\ell)}(\mathbf{R})\in \mathbb C^{(2\ell_1+1)\times(2\ell_2+1)}$ is the Wigner D-matrix.


By substituting above \cref{eq:app_te_transform} in \cref{eq:tensor_expansion}, the entry of rotated tensor expansion is
\begin{equation}
    \left(\bar{\otimes} \mathbf{w}^{(\ell)}  \right)^{(\ell_1,\ell_2)}_{(m_1,m_2)} \xrightarrow{\mathbf{R}}
    \left( \bar{\otimes} \left[\mathbf{R}\cdot \mathbf{w}^{(\ell)}\right] \right)=
    \sum_{m} C_{(\ell_1,m_1),(\ell_2,m_2)}^{(\ell,m)} \left[\sum_{m'} D^{(\ell)}_{m m'}(\mathbf{R}) w^{(\ell)}_{m'}\right],
\end{equation}
and we can exchange the order of summation:
\begin{equation}
    \left(\bar{\otimes} \mathbf{w}^{(\ell)}  \right)^{(\ell_1,\ell_2)}_{(m_1,m_2)} \xrightarrow{\mathbf{R}}
     \sum_{m'}\left(\sum_{m} C_{(\ell_1,m_1),(\ell_2,m_2)}^{(\ell,m)} D^{(\ell)}_{m m'}(\mathbf{R}) \right)w^{(\ell)}_{m'}.
\end{equation}

Now we can use a crucial identity from representation theory: 
\begin{theorem}
The Clebsch–Gordan coefficients provide a basis change between the product representation  $D^{(\ell_1)}(\mathbf{R}) \otimes D^{(\ell_2)}(\mathbf{R})$  and the irreducible representation  $D^{(\ell)}(\mathbf{R})$:
\begin{equation}
    \sum_{m} C_{(\ell_1,m_1),(\ell_2,m_2)}^{(\ell,m)} D^{(\ell)}_{m m'}(\mathbf{R}) = \sum_{m_1',m_2'} D^{(\ell_1)}_{m_1 m_1'}(\mathbf{R}) D^{(\ell_2)}_{m_2m_2'}(\mathbf{R}) C_{(\ell_1,m_1'),(\ell_2,m_2')}^{(\ell,m')}.
\end{equation}

\end{theorem}
We can substitute the identity, then we have:
\begin{equation}
    \left(\bar{\otimes} \mathbf{w}^{(\ell)}  \right)^{(\ell_1,l_2)}_{(m_1,m_2)} \xrightarrow{\mathbf{R}}
     \sum_{m_1',m_2'}
     D^{(\ell_1)}_{m_1 m_1'}(\mathbf{R})
     D^{(\ell_2)}_{m_2m_2'}(\mathbf{R})
     \left(\sum_{m'}C_{(\ell_1,m_1'),(\ell_2,m_2')}^{(\ell,m')} w^{(\ell)}_{m'}\right),
\end{equation}
and the last sum implies the
\begin{equation}
    \sum_{m'}C_{(\ell_1,m_1'),(\ell_2,m_2')}^{(\ell,m')} w^{(\ell)}_{m'} = \left(\bar{\otimes} \mathbf{w}^{(\ell)}  \right)^{(\ell_1,\ell_2)}_{(m_1',m_2')}
\end{equation}

Therefore,
\begin{equation}
    \left(\bar{\otimes} \mathbf{w}^{(\ell)}  \right)^{(\ell_1,\ell_2)}_{(m_1,m_2)}
    \xrightarrow{\mathbf{R}}
     \sum_{m'_1,m'_2}
     D^{(\ell_1)}_{m_1 m_1'}(\mathbf{R})
     D^{(\ell_2)}_{m_2 m_2'}(\mathbf{R})
     \left(\bar{\otimes}\mathbf{w}^{(\ell_3)}  \right)^{(\ell_1,\ell_2)}_{(m_1',m_2')},
\end{equation}

in the matrix form,
\begin{equation}
    \left(\bar{\otimes} \mathbf{w}^{(\ell)}  \right) \xrightarrow{\mathbf{R}} D^{(\ell_1)}(\mathbf{R})\left(\bar{\otimes} \mathbf{w}^{(\ell)}  \right) D^{(\ell_2)}(\mathbf{R})^{-1}.
\end{equation}

\subsection{Proof of the invariance of the tensor expansion based (TE) prior}
\label{app:proof_tensor_invariance}

To construct an SO(3)-invariant distribution over matrices via tensor expansion, we begin with a rotationally invariant distribution over irreducible features $ \mathbf{w}^{(\ell)} \in \mathbb{C}^{(2\ell+1)} $. We define this distribution by factorizing it into two independent components:
\begin{itemize}
    \item A magnitude $ r = \|\mathbf{w}^{(\ell)}\| $ drawn from a radial distribution, e.g., $ r \sim \text{Normal}(1, \sigma^2) $.
    \item A direction sampled uniformly on the sphere $ \mathbb{S}^{2} $, induced by a Haar-uniform rotation $ \mathbf{R} \in \text{SO(3)} $, applied to a canonical unit-norm feature vector $ \mathbf{w}_0^{(\ell)} $, such that $ \mathbf{w}^{(\ell)} = rD^{(\ell)}(\mathbf{R})\, \mathbf{w}_0^{(\ell)} $.
\end{itemize}

This construction ensures that $ \mathbf{w}^{(\ell)} $ is distributed isotropically, i.e., $ p(\mathbf{w}^{(\ell)}) = p(D^{(\ell)}(\mathbf{R})\mathbf{w}^{(\ell)}) $ for any $ \mathbf{R} \in \text{SO(3)} $. Now, from the tensor expansion defined as:
\begin{equation}    
    \mathbf{H}^{(\ell_1,\ell_2)} = \left(\bar{\otimes} \mathbf{w}^{(\ell)}\right)^{(\ell_1,\ell_2)},
\end{equation}

we know from the previous subsection that this construction transforms under SO(3) as:
\begin{equation}    
    \mathbf{H}^{(\ell_1,\ell_2)} \xrightarrow{\mathbf{R}} D^{(\ell_1)}(\mathbf{R}) \mathbf{H}^{(\ell_1,\ell_2)}D^{(\ell_2)}(\mathbf{R})^{-1}.
\end{equation}

To prove invariance, consider the pushforward distribution:
\begin{equation}
    p(\mathbf{H}^{(\ell_1,\ell_2)}) = p(\mathbf{w}^{(\ell)}) = p(D^{(\ell)}(\mathbf{R})\mathbf{w}^{(\ell)}) \quad \forall \mathbf{R} \in \text{SO(3)}.
\end{equation}

Because $ \mathbf{H}^{(\ell_1,\ell_2)} $ is a deterministic, equivariant function of $ \mathbf{w}^{(\ell)} $, and $ p(\mathbf{w}^{(\ell)}) $ is rotation-invariant, the induced distribution $ p(\mathbf{H}^{(\ell_1,\ell_2)}) $ must also be invariant under conjugation by $ D^{(\ell_1)}(\mathbf{R}) $ and $D^{(\ell_2)}(\mathbf{R})$. Thus:
\begin{equation}
    p(\mathbf{H}^{(\ell_1,\ell_2)}) = p(D^{(\ell_1)}(\mathbf{R})\, \mathbf{H}^{(\ell_1,\ell_2)}\, D^{(\ell_2)}(\mathbf{R})^{-1}).
\end{equation}
This proves that the prior distribution constructed via tensor expansion from rotationally invariant $ \mathbf{w}^{(\ell)} $ yields an SO(3)-equivariant (conjugation-invariant) distribution over matrix-valued outputs.

\subsection{Proof of the invariance of the multiple tensor expansion prior}
\label{app:proof_tensor_expansion_multi}

We now generalize the single-irrep vector expansion to construct a full Hamiltonian matrix $ \mathbf{H} \in \mathbb{R}^{n \times n} $ composed of multiple  irrep vectors components. Let the atomic orbital basis consist of a set of irrep vectors indexed by $ L = \{\ell_1, \ell_2, \dots, \ell_B\} $, where each angular momentum $ \ell_i $ corresponds to a subspace of dimension $(2\ell_i + 1)$.

For each irrep vector rank $ \ell_i $, we define a random irrep vector $ \mathbf{w}^{(\ell_i)} \in \mathbb{C}^{(2\ell_i+1)} $, sampled independently from a rotationally invariant distribution:
\begin{equation}
\mathbf{w}^{(\ell_i)} = r_i  D^{(\ell_i)}(\mathbf{R}_i) \mathbf{w}_0^{(\ell_i)}, \quad r_i \sim \text{LogNormal}(1, \sigma^2), \quad \mathbf{R}_i \sim \text{Uniform}(\text{SO(3)}).
\end{equation}
We then define a factorized prior:
\begin{equation}
    p(\mathbf{w}^{(\ell_1)}, \ldots, \mathbf{w}^{(\ell_B)}) = \prod_{i=1}^B p_i(\mathbf{w}^{(\ell_i)}),
\end{equation}
with each $ p_i(\mathbf{w}^{(\ell_i)}) $ being SO(3)-invariant.

Using the tensor expansion, each pair $ (\ell_i, \ell_j) $ generates a block of the Hamiltonian matrix via:
\begin{equation}
    \mathbf{H}^{(\ell_i, \ell_j)} = \bar{\otimes}_{\ell_i, \ell_j} \mathbf{w}^{(\ell_k)}, \quad \text{for some } \ell_k \in \{|\ell_i - \ell_j|, \dots, \ell_i + \ell_j\}.
\end{equation}
The full Hamiltonian is then assembled as:
\begin{equation}    
    \mathbf{H} = \bigoplus_{i,j} \mathbf{H}^{(\ell_i, \ell_j)}.
\end{equation}
From the single-component proof, we know that each block transforms as:
\begin{equation}
    \mathbf{H}^{(\ell_i,\ell_j)}
    \xrightarrow{\mathbf{R}}
    D^{(\ell_i)}(\mathbf{R})
    \mathbf{H}^{(\ell_i,\ell_j)}
    D^{(\ell_j)}(\mathbf{R})^{-1}.
\end{equation}
Therefore, under a global rotation $ \mathbf{R} \in \text{SO(3)} $, the full matrix $ \mathbf{H} $ transforms as:
\begin{equation}
    \mathbf{H} \xrightarrow{\mathbf{R}} \mathcal{D}(\mathbf{R}) \, \mathbf{H} \, \mathcal{D}(\mathbf{R})^{-1},
\end{equation}
where $ \mathcal{D}(\mathbf{R})$ is the block-diagonal rotation operator acting on the full basis.

Since each $ \mathbf{w}^{(\ell_i)} $ is sampled independently from an SO(3)-invariant distribution, the joint distribution of all irreducible components $ p(\mathbf{H}) $ remains invariant under this global conjugation:
\begin{equation}
    p(\mathbf{H}) = p\left(\mathcal{D}(\mathbf{R}) \, \mathbf{H} \, \mathcal{D}(\mathbf{R})^{-1}\right), \quad \forall \mathbf{R} \in \text{SO(3)}.
\end{equation}
This completes the proof that the full Hamiltonian matrix constructed via multiple tensor expansions, using independently sampled spherical features from invariant priors, defines an SO(3)-invariant distribution over matrices.

\clearpage
\section{Implementation details}

\subsection{Model implementation}
\label{app:model_implementation}

We build our model upon the official QHNet~\cite{yu2023efficient} and DEQHNet~\cite{wanginfusing} codebases, which implement SE(3)-equivariant GNN for Hamiltonian matrix prediction. QHNet is selected as our backbone for its balance of architectural simplicity and strong predictive performance. Although more recent models such as WANet~\cite{lienhancing} and SPHNet~\cite{luo2025efficient} have demonstrated improvements, their codebases are not publicly available and thus are not considered here. Notably, our method is model-agnostic and could be paired with more expressive backbones if desired.

We extend QHNet by incorporating additional physically meaningful inputs: the current Hamiltonian matrix $\mathbf{H}_t$, the overlap matrix $\mathbf{S}$, the molecular configuration $\mathcal{M}$, and the time $t$. Unlike the original QHNet, which processes only $\mathcal{M}$, our model is designed to handle $\mathbf{H}_t$, and $\mathbf{S}$ as well, following symmetry-preserving strategies inspired by DEQHNet and OrbNet-Equi~\cite{qiao2020orbnet}.

\textbf{Project Block.} To map the equivariant matrix features $\mathbf{H}$ and $\mathbf{S}$ into the SO(3) irrep vectors, we used \textit{diagonal reduction} in OrbNet~\cite{qiao2020orbnet} based on the Wigner-Eckart theorem~\cite{wigner1993matrices}. For atom $i$, we first extract the atom-wise matrices, $\mathbf{H}_i\coloneq\mathbf{H}_{ii}$ (see \cref{eq:atomwise_ham}). Each element of $\mathbf{H}_i$ carries two orbital index, $(\ell,m)$ and $(\ell',m')$. We project these matrices onto rank-$\ell_{\text{o}}$ irrep vectors $\mathbf h^{(\ell_{\text{o}})}_i=[h^{(\ell_{\text{o}},-\ell_{\text{o}})}_i,\ldots h^{(\ell_{\text{o}},\ell_{\text{o}})}_i] \in \mathbb C^{(2\ell_{\text{o}} +1)}$ by
\begin{equation}
    {h}_i^{(\ell_{\text{o}},m_{\text{o}})} = \sum_{(\ell,\ell')} \sum_{(m,m')} \mathbf{H}_{i}^{(\ell,m; \ell',m')} Q^{(\ell,m; \ell',m')}_{i,(\ell_{\text{o}},m_{\text{o}})},
    \label{eq:diag_reduce}
\end{equation}
where $\mathbf{H}_{i}^{(\ell,m; \ell',m')}$ is an element of submatrix $\mathbf{H}_{i}^{(\ell,\ell')}$ that corresponds to the $m$ and $m'$ index, and a set of atom-wise projection weights $Q^{(\ell,m; \ell',m')}_{i, (\ell_{\text{o}},m_{\text{o}})}$ which plays the role of Clebsch-Gordan-like projection weights. Because the map in \cref{eq:diag_reduce} is an SO(3) tensor contraction, the resulting feature vectors remain equivariant. The same procedure is applied to overlap matrix $\mathbf{S}$, giving two parallel streams of SE(3)-equivariant atomic features that are subsequently fused in the network.

\textbf{Construction of projection weights.} 
To construct the coefficients atom-wise projection coefficients, we compute three-center integrals involving orbital basis function $\Phi^{(\ell,m)}_i$ and auxiliary spherical-type basis functions $\tilde{\Phi}^{(l,m)}_i$:
\begin{equation}
    Q^{(\ell,m; \ell',m')}_{i, (\ell_{\text{o}},m_{\text{o}})} = \int \left( \Phi_i^{(\ell,m)}(\mathbf{r}) \right)^* \Phi_i^{(\ell',m')}(\mathbf{r}) \tilde{\Phi}_i^{(\ell_{\text{o}},m_{\text{o}})}(\mathbf{r}) \, d\mathbf{r}.
\end{equation}
In practice, the angular parts of these integrals are related with the Clebsch-Gordan coefficients due to their relation to spherical harmonics:
\begin{equation}
     Q^{(\ell,m; \ell',m')}_{i, (\ell_{\text{o}},m_{\text{o}})} \propto \int_{\mathbb{S}^2} Y^{\ell}_{m}(\hat{\mathbf{r}}) Y^{\ell'}_{m}(\hat{\mathbf{r}}) \bigl(Y^{\ell_\text{o}}_{m_\text{o}}(\hat{\mathbf{r}})\bigr)^*d\mathbf{r}.
\end{equation}
\subsection{Training objective}
\label{sec:training_objective}

Our training objective adopts a residual learning strategy, following prior works such as WANet and SHNet. Rather than directly predicting the converged Hamiltonian, the model learns to approximate the residual between the initial and converged Hamiltonians using a time-dependent vector field within the conditional flow matching framework. We define the residual target as done in prior works:
\begin{equation}
\mathbf{H}_{1,\mathcal{M}} := \mathbf{H}^{\star}_{\mathcal{M}} - \mathbf{H}^{(0)}_{\mathcal{M}},
\end{equation}
 where $\mathbf{H}^{(0)}_{\mathcal{M}}$ is the initial guess of Hamiltonian matrix\footnote{We use the \texttt{minao} initialization from the \texttt{PySCF} package, and this guess does not contains SCF steps.}, and $\mathbf{H}^{\star}_{\mathcal{M}}$ is the SCF solution. The final prediction of Hamiltonian is obtained by summing the predicted residual and the initial Hamiltonian guess.

The conditional flow matching loss is defined as:
\begin{align}
\mathcal{L}
&= \mathbb{E}_{(\mathbf{H}, \mathcal{M})\sim \mathcal{A}, t \sim \mathcal{U}(0,1), \mathbf{H}_{t} \sim p_{t}} \left[\left\| v_{t,\theta}(\mathbf{H}_{t,\mathcal{M}}) - u_t(\mathbf{H}_{t,\mathcal{M}} \mid \mathbf{H}_{1,\mathcal{M}}) \right\|^2_2 \right] \\
&= \mathbb{E}_{(\mathbf{H}, \mathcal{M})\sim \mathcal{A}, t \sim \mathcal{U}(0,1), \mathbf{H}_{t} \sim p_{t}} \left[\frac{1}{(1 - t)^2} \left\| \mathbf{H}_{1,\mathcal{M}}^{(\theta)} - \mathbf{H}_{1,\mathcal{M}} \right\|^2_2 \right],
\end{align}

where the second line follows from the analytical form of the conditional velocity field $u_t$, showing that the model is penalized based on the squared residual error at each time step. This formulation encourages smooth convergence from the initial guess to the target solution. To simplify the objective, we omit the $1/(1-t)^2$ time-scaling for our implementation.


\clearpage
\section{Experimental study settings}
\label{app:experiment_setting}
\subsection{Dataset preparation}
\label{app:dataset}
To demonstrate the effectiveness of flow-matching-based training, we conduct experiments on two molecular datasets: MD17 and QH9. The MD17 represents a relatively simple task compared to the QH9, focusing solely on small systems and their conformational space. The PubChemQH9 is not considered since their dataset and codebase are not publicly released.

\textbf{MD17.} 
The MD17~\cite{chmiela2017machine,schutt2019unifying} dataset consists of quantum chemical simulations for four small organic molecules: water (\ce{H2O}), ethanol (\ce{C2H5OH}), malondialdehyde (\ce{CH2(CHO)2}), and uracil (\ce{C4H4N2O2}). It provides a comprehensive set of molecular properties, including geometries, total energies, forces, Kohn–Sham Hamiltonian matrices, and overlap matrices. All reference computations were implemented via the ORCA electronic structure package~\cite{neese2020orca} using the PBE exchange–correlation functional~\cite{perdew1996generalized,weigend2005balanced} and the def2-SVP Gaussian-type orbital (GTO) basis set. We follow the standard data split protocol used in prior work~\cite{schutt2019unifying,unke2021se,yu2023efficient} to divide each molecule’s conformational data into training, validation, and test sets. The detailed dataset statistics are summarized in \cref{tab:md17_stats} and MOs in the table imply molecular orbitals (\textit{i.e.}. s,p,d,f)

\begin{table}[h]
\centering
\caption{The statistics of MD17 dataset~\cite{schutt2019unifying}.}
\label{tab:md17_stats}
\resizebox{\textwidth}{!}{
\begin{tabular}{lrrrrrrr}
\toprule
\textbf{Dataset} & \textbf{\# of structures} & \textbf{Train} & \textbf{Val} & \textbf{Test} & \textbf{\# of atoms} & \textbf{\# of orbitals} & \textbf{\# of occupied MOs} \\
\midrule
\midrule
Water            & 4,900     & 500   & 500   & 3,900  & 3   & 24  & 5  \\
Ethanol          & 30,000    & 25,000 & 500  & 4,500  & 9   & 72  & 10 \\
Malondialdehyde  & 26,978    & 25,000 & 500  & 1,478  & 9   & 90  & 19 \\
Uracil           & 30,000    & 25,000 & 500  & 4,500  & 12  & 132 & 26 \\
\bottomrule
\end{tabular}
}
\end{table}


\textbf{QH9.} The QH9 dataset~\cite{yu2023qh9} is a large-scale quantum chemistry benchmark designed to support the training and evaluation of machine learning models for Hamiltonian matrix prediction across diverse chemical structures. It is based on the QM9~\cite{ruddigkeit2012enumeration,ramakrishnan2015electronic} molecular dataset and includes 130,831 Hamiltonian matrices from stable molecular geometries, as well as 2,698 molecular dynamics trajectories. The dataset covers small organic molecules composed of up to nine heavy atoms (C, N, O, and F). All Hamiltonians were computed using the PySCF~\cite{sun2018pyscf} quantum chemistry package with the B3LYP~\cite{stephens1994ab} exchange–correlation functional and the def2-SVP Gaussian-type orbital (GTO) basis set. We provide the detailed dataset statistics in \cref{tab:qh9_stats}.


QH9 is organized into two main subsets, QH9-\texttt{stable} and \texttt{QH9-dynamic-300k}, and provides four standard evaluation splits: stable-\texttt{id}, stable-\texttt{ood}, dynamic-300k-\texttt{geo}, and dynamic-300k-\texttt{mol}. The \texttt{id} split randomly partitions the \texttt{QH9-stable} subset into training, validation, and test sets, while the \texttt{ood} split is constructed based on molecular size. Specifically, it groups molecules with 3–20 atoms in the training set, molecules with 21–22 atoms in the validation set, and molecules with 23–29 atoms in the test set. This \texttt{ood} setup allows for a rigorous evaluation of out-of-distribution (OOD) generalization in terms of molecular complexity.

The \texttt{geo} and \texttt{mol} splits are based on molecular dynamics (MD) trajectories, where each molecule is associated with 100 geometry snapshots. In the \texttt{geo} split, geometries are randomly assigned within each molecule: 80 for training, 10 for validation, and 10 for testing. Thus, while all molecules are present across the splits, the specific conformations are disjoint, enabling an assessment of geometric generalization. In contrast, the \texttt{mol} split divides the 2,698 molecules themselves into disjoint sets with an 80/10/10 train/validation/test ratio. All 100 geometries of a molecule are assigned to the same subset. This split presents a more challenging task than the \texttt{geo} split, as it requires generalization to entirely unseen molecular identities rather than just new conformations.

\begin{table}[h]
\centering
\caption{The statistics of QH9 dataset \cite{yu2023qh9}.}
\label{tab:qh9_stats}
\begin{tabular}{lrrrrr}
\toprule
\textbf{Dataset} & \textbf{\# of structures} & \textbf{\# of Molecules} & \textbf{Train} & \textbf{Val} & \textbf{Test} \\
\midrule
\midrule
Stable-id         & 130,831   & 130,831       & 104,664 & 13,083  & 13,084     \\
Stable-ood         & 130,831   & 130,831       & 104,001 & 17,495  & \ptz9,335  \\
Dynamic-300k-geo   & 269,800   & \ptz\ptz2,698 & 215,840 & 26,980  & 26,980     \\
Dynamic-300k-mol   & 269,800   & \ptz\ptz2,698 & 215,800 & 26,900  & 27,100     \\
\bottomrule
\end{tabular}
\end{table}

\subsection{Evaluation Metrics}
\label{app:metric}
To comprehensively evaluate the performance of Hamiltonian prediction models, we adopt several metrics that measure accuracy, physical fidelity, and downstream impact on quantum chemical properties. Below are detailed descriptions of each metric used in our experiments.

\textbf{Hamiltonian MAE.} This metric measures the mean absolute error (MAE) between the predicted Hamiltonian matrix $\hat{\mathbf{H}}$ and the ground-truth matrix $\mathbf{H}^\star$:
\begin{equation}
\operatorname{MAE}({\mathbf{H}}) = \frac{1}{n^2} \sum_{i,j=1}^{n} \left\| \hat{\mathbf{H}}_{ij} - \mathbf{H}^\star_{ij} \right\|^2_2,
\end{equation}
where $n$ is the length of the Hamiltonian matrix ($\mathbf H \in \mathbb R^{n\times n}$), and $\|\cdot\|^2_2$ is the Frobenius norm. This metric directly reflects the quality of the predicted Hamiltonian in element-wise terms.

\textbf{Occupied orbital energy MAE (\OCC).}
This metric measures the MAE between the predicted and true orbital energies for only the occupied orbitals. Let $\hat{{\epsilon}}$ and ${\epsilon}^\star$ be predicted and the ground-truth generalized eigenvalues of the Hamiltonian, respectively, and let $\mathcal I_\text{occ}$ be the set of indices of the occupied orbitals:
\begin{equation}
\operatorname{MAE}({\epsilon_\text{occ}}) = \frac{1}{\operatorname{card}(\mathcal I_\text{occ})} \sum_{i \in \mathcal I_\text{occ} } \left\| \hat{\epsilon}_i - \epsilon^\star_i \right\|^2_2.
\end{equation}
This is particularly important for capturing the energy spectrum relevant to ground-state electronic properties. We identify the occupied orbitals by selecting the $\lfloor{N}/{2}\rfloor$ lowest eigenvalues, where $N$ is the number of electrons in the system.

\textbf{Orbital coefficient similarity score (\SC).}
To compare the predicted and ground-truth molecular orbital coefficient matrices $\hat{\mathbf{C}}$ and $\mathbf{C}^\star$, we use a cosine similarity-based score averaged over all columns:
\begin{equation}
\mathcal S_C(\hat{\mathbf C},\mathbf C^\star) = \left\langle \hat{\mathbf{C}}, \mathbf{C}^\star \right\rangle=\frac{\sum_i\mathbf{C}_i\mathbf{C}^\star_i}{\|\hat{\mathbf{C}}\|\|\mathbf{C}^\star\|},
\end{equation}
where $\mathbf{C}_i$ is the $i$-th column vector of the coefficient matrix and $\langle \cdot, \cdot \rangle$ denotes the inner product. This metric evaluates how well the predicted orbitals align with the ground truth.

\textbf{HOMO, LUMO, and energy gap MAE (\HOMO, \LUMO, \GAP).}
These metrics quantify the predictive accuracy of specific frontier orbital energies, which are critical for determining electronic properties such as reactivity and charge transport. The highest occupied molecular orbital (HOMO) and lowest unoccupied molecular orbital (LUMO) energies, along with their difference (the HOMO–LUMO gap), are particularly sensitive to model generalization, especially in challenging settings like QH9, where predictions are evaluated on unseen molecular structures or conformations. These metrics are computed as follows:
\begin{align}
\epsilon_\text{HOMO} &= \left| \hat{\epsilon}_{\text{HOMO}} - \epsilon^\star_{\text{HOMO}} \right|, \\
\epsilon_\text{LUMO} &= \left| \hat{\epsilon}_{\text{LUMO}} - \epsilon^\star_{\text{LUMO}} \right|, \\
\epsilon_\Delta  &= \left| (\hat{\epsilon}_{\text{LUMO}} - \hat{\epsilon}_{\text{HOMO}}) - (\epsilon^\star_{\text{LUMO}} - \epsilon^\star_{\text{HOMO}}) \right|.
\end{align}
Here, $\epsilon_\text{HOMO}$ corresponds to the $\lfloor N/2 \rfloor$-th lowest eigenvalue, and $\epsilon_\text{LUMO}$ to the $(\lfloor N/2 \rfloor + 1)$-th, where $N$ is the number of electrons in the system.

\textbf{SCF \texttt{Iter} Ratio}:
This metric measures the reduction in the number of SCF iterations required when using a predicted Hamiltonian as the initial guess, relative to a standard reference initialization (e.g., from a minimal basis or atomic superposition guess). It is defined as
\begin{equation}
    \text{SCF \texttt{Iter} Ratio} = \frac{\texttt{Iter}_{\text{pred}}}{\texttt{Iter}_{\text{ref}}},
\end{equation}
where $\texttt{Iter}_{\text{pred}}$ is the number of SCF iterations with the predicted initialization, and $\texttt{Iter}_{\text{ref}}$ is the number of iterations under the reference setup. In our setting, we used the reference value, which is measured from the conventional DFT metric to compare the acceleration of our method.

\textbf{SCF \texttt{T} Ratio}:
This represents the reduction in total wall-clock time spent during SCF convergence using the predicted Hamiltonian. It reflects actual runtime savings in quantum chemical simulations:
\begin{equation}
    \text{SCF \texttt{T} Ratio} = \frac{T_{\text{SCF-pred}}}{T_{\text{SCF-ref}}},
\end{equation}
where $T_{\text{SCF-pred}}$ and $T_{\text{SCF-ref}}$ denote the SCF runtimes under predicted and reference initializations, respectively.

\textbf{Inf \texttt{T} Ratio}:  
This metric captures the inference overhead of the predictive model itself. It is the fraction of time required to generate the predicted Hamiltonian relative to the baseline SCF time:
\begin{equation}
    \text{Inf \texttt{T} Ratio} = \frac{T_{\text{inference}}}{T_{\text{SCF-ref}}},
\end{equation}
where $T_{\text{inference}}$ is the runtime of the Hamiltonian prediction model.

\textbf{Total \texttt{T} Ratio}:  
This quantifies the net cost of using the predictive model, combining both inference and SCF convergence times. It provides a holistic view of overall computational efficiency:
\begin{equation}
\text{Total \texttt{T} Ratio} = \frac{T_{\text{inference}} + T_{\text{SCF-pred}}}{T_{\text{SCF-ref}}}.
\end{equation}

\textbf{Note.} All energy values are reported in units of Hartree ($1E_h=27.211 eV$), and similarity scores are unitless with values in $[0, 1]$, where higher is better. While the SCF \texttt{Iter} Ratio is a deterministic metric reflecting algorithmic convergence behavior, the wall-clock timing ratios (SCF \texttt{T}, Inf \texttt{T}, and Total \texttt{T}) are subject to variability due to system-level factors. In our experiments, all timing evaluations were conducted on A100-80GB GPUs. However, due to resource allocation via SLURM and shared CPU environments, precise time measurements were not always reproducible. As such, reported time ratios should be interpreted as indicative trends rather than absolute benchmarks.

\subsection{Experimental setup}

\textbf{Environment.} Experiments were conducted using a single GPU per model. For the MD17 dataset, we used NVIDIA RTX 3090 and A5000 GPUs, while for the QH9 dataset, experiments were performed on NVIDIA A100 80GB GPUs.
Our implementation is based on PyTorch 2.1.2 and PyG 2.3.0, both compiled with CUDA 12.1. Detailed package versions~\cite{sun2018pyscf,geiger2022e3nn,larsen2017atomic} and environment specifications will be released upon publication for full reproducibility.

Training was performed on a SLURM-managed cluster, where slight variability in runtime was observed due to system-wide GPU and CPU resource contention. Random seeds were fixed where possible to ensure training stability; however, minor non-determinism remains due to the inherent variability of distributed computing environments.

Training QHFlow took approximately 2–4 days on MD17 and 7–10 days on QH9, which is slightly longer than QHNet due to the added complexity of incorporating the current Hamiltonian and orbital information as inputs. Finetuning on QH9 required an additional 3–4 days. While the total training time could be further reduced with optimized infrastructure, our experiments were conducted under a SLURM-managed environment with periodic reinitialization every 72 hours. Importantly, QHFlow is a model-agnostic framework; with more scalable architectures, training efficiency can be significantly improved.

\textbf{Hyperparameters.}  
For fair comparison, we adopted the same hyperparameters used by the baseline model QHNet~\cite{yu2023efficient} whenever possible. Our QHFlow shares the majority of its architecture and training settings with QHNet to ensure that performance improvements are attributable to the proposed flow matching design rather than hyperparameter tuning. A summary of the key hyperparameters used across different datasets is provided in \cref{tab:hyperparams}.

\begin{table}[h]
\centering
\caption{Training hyperparameters of QHFlow used across datasets.}
\label{tab:hyperparams}
\resizebox{\textwidth}{!}{
\begin{tabular}{llccc}
\toprule
\textbf{Hyperparameter} & \textbf{Description} & \textbf{QH9} & \textbf{MD17 (Water)} & \textbf{MD17 (Others)} \\
\midrule
\midrule
Learning Rate & Initial learning rate
& 1e-3 & 5e-4 & 1e-3 \\
Minimum Learning Rate & Minimum learning rate
& 1e-7 & 1e-9 & 1e-9 \\
Batch Size & Number of molecules per batch
& 32 & 10 & 5 \\
Scheduler & Learning rate scheduler
& Polynomial & Polynomial & Polynomial \\
LR Warmup Steps & Warmup steps to linearly increase learning rate
& 1,000 & 1,000 & 1,000 \\
Max Steps & Maximum number of training steps
& 260,000 & 200,000 & 200,000 \\
Fine-tuning LR & Initial learning rate of fine-tuning stage
& 1e-5 & - & - \\
Fine-tuning Minimum LR & Minimum learning rate of fine-tuning stage
& 1e-7 & - & - \\
Finetuning Steps & Maximum number of Finetuning steps
& 60,000 & - & - \\
Prior Distribution & Prior distribution for flow matching
& GOE / TE & GOE & GOE \\
Using $H_t$ Block & Use time-dependent Hamiltonian $H_t$ as input
& True & True & True \\
Using $S$ Block & Use overlap matrix $S$ as input
& True & False & False \\
Model Order & Maximum degree of spherical harmonics
& 4 & 4 & 4 \\
Embedding Dimension & Node feature embedding dimension
& 128 & 128 & 128 \\
Bottle Hidden Size & Hidden size of bottleneck layer
& 32 & 32 & 32 \\
Number of GNN Layers & Number of graph neural network layers
& 5 & 5 & 5 \\
Max Radius & Cutoff radius for neighbor search
& 15 & 15 & 15 \\
Sphere Channels & Number of channels in spherical basis
& 128 & 128 & 128 \\
Edge Channels & Number of channels for edge features
& 32 & 32 & 32 \\
\bottomrule
\end{tabular}
}
\end{table}


\clearpage
\section{Additional experimental results and limitations}

\subsection{Ablation study of the finetuning objective.}
\label{app:finetune_additional}

We conduct additional experiments to evaluate various fine-tuning strategies to improve the Hamiltonian prediction performance of QHFlow after standard flow matching pretraining. In this section, we describe each strategy in detail and provide empirical observations.

For the WALoss implementation, we follow the coefficient settings proposed in WANet~\cite{lienhancing} ($\lambda_{\text{WA}}=2.0$). During fine-tuning, we train for an additional 60,000 steps starting from the pretrained model with TE prior, using an initial learning rate of $1\times10^{-5}$ and a polynomial learning rate scheduler.

\textbf{Full FM + WA Loss training from scratch (WA-Full).}
In this strategy, we train the model from scratch by jointly optimizing the flow matching objective and WALoss for 260,000 steps, matching the default training steps as done in WANet. However, this approach significantly degraded the Hamiltonian error. We hypothesize that imposing strong spectral constraints too early disrupts the learning of the global Hamiltonian structure, leading to unstable convergence and poor generalization.

\textbf{WA Loss finetuning (WA-FT).}
After completing standard flow matching pre-training, we fine-tune the model solely using WALoss, which encourages alignment between the predicted Hamiltonian's eigenstructure and the ground-truth SCF solutions. This approach improves orbital energy prediction and SCF convergence compared to pure flow matching training, confirming the value of adding spectral supervision during fine-tuning.


\textbf{Summary.}
\cref{tab:qh9_finetunes} summarizes the quantitative results of all fine-tuning strategies. Here, w/o-FT refers to QHFlow trained solely with the flow matching objective using the TE prior. Among the approaches, WA-FT achieves the best balance between Hamiltonian prediction accuracy and practical DFT acceleration, demonstrating the effectiveness of spectral alignment in the fine-tuning stage.


\subsection{Full results of ablation study}
\label{app:full_ablation}

For completeness, we provide the full ablation study results in \cref{tab:qh9_dist_full}, and \cref{tab:qh9_variance}, including additional metrics beyond those presented in the main text. While the main manuscript focused primarily on Hamiltonian prediction error ($H$), occupied orbital energy error (\OCC), and electronic density accuracy (\SC) for clarity, here we also report the LUMO (\LUMO), HOMO (\HOMO), and HOMO-LUMO gap (\GAP) energy errors.

Overall, the trends observed in the full table are consistent with those discussed in the main text. In particular, the improvements in Hamiltonian accuracy and density prediction are accompanied by consistent reductions in orbital energy errors (\LUMO, \HOMO) and gap errors (\GAP), further demonstrating the broad effectiveness of our proposed methods. These results reinforce the conclusion that flow matching enhance both Hamiltonian structure prediction and downstream electronic properties.

Also, to better visualize the role of the prior distributions, we provide interpolation trajectories from the GOE and TE prior toward target Hamiltonians. \cref{fig:prior_interpolation} shows example interpolations for both settings, highlighting how the initial distribution affects the learned flow dynamics.  As seen, the TE prior results in smoother and more structured trajectories compared to the GOE prior, which starts from unstructured noise.

\input{table/qh9_finetuning}
\input{table/qh9_distribution_full}
\input{table/qh9_variance}

\begin{figure}[t]
    \centering
    \includegraphics[width=1\linewidth]{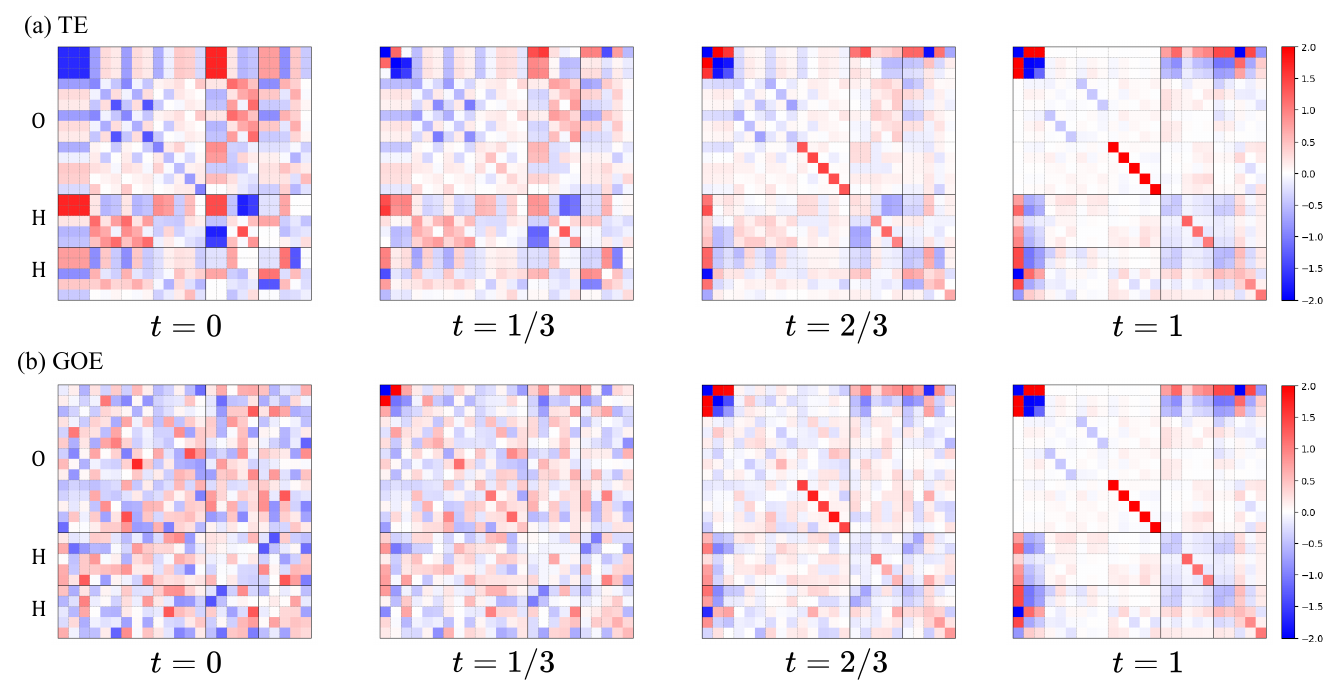}
    \caption{Visualization of Hamiltonian interpolation trajectories from different prior distributions of \ce{H2O}: (a) tensor expansion-based (TE) prior and (b) Gaussian orthogonal ensemble (GOE) prior. Color intensity indicates the magnitude of Hamiltonian elements across flow time $ t $.
}
    \label{fig:prior_interpolation}
\end{figure}

\subsection{Analysis of error distribution of the predictions}

To better understand the properties of \QHFlow{}, we move beyond single–number summaries and visualise the entire error distribution for six key quantities Hamiltonian MAE ($H$), occupied–orbital MAE ($\epsilon_{\text{occ}}$), \HOMO, \LUMO, \GAP, and \SC{} on all four QH9 splits (\texttt{id}, \texttt{ood}, \texttt{geo}, \texttt{mol}).
\cref{fig:prop_violin} shows log-scale violin plots for QHNet* (grey), \QHFlow{} (orange), and its WA-finetuned variant (cyan). (only the similarity score is kept on a linear axis.) Each violin displays the full empirical distribution; the thick dashed line marks the median, and the two thinner lines divide the inter-quartile ranges.

Across every split and metric, the \QHFlow{} violins are both \emph{lower} and \emph{narrower}.
Median Hamiltonian error is reduced by roughly one order of magnitude on \texttt{id} and \texttt{geo}, and by a factor of~3–5 on the tougher \texttt{ood} and \texttt{mol} sets.
In addition, the long error tails of QHNet* largely vanish, demonstrating that our flow objective mitigates the occasional catastrophic failure modes that plague point-wise regression models.

\cref{fig:HvE} plots $\log H$ against $\log\epsilon_{\text{occ}}$ for every test geometry.
\QHFlow{} occupies the bottom-left corner of each panel, while QHNet* points fan out towards larger joint errors, especially in \texttt{ood} and \texttt{mol}, where chemical diversity is highest. These results show the \QHFlow{} superior performance on both the geometric and unseen molecules.

Finally, \cref{fig:NvH} compares Hamiltonian error versus atom count. \QHFlow{} remains flat up to the largest molecules in QH9 (29atoms). This suggests that modeling a \emph{distribution} over Hamiltonians confers a form of size transferability.

\begin{figure}[t]
    \centering
    \includegraphics[width=1.0\linewidth]{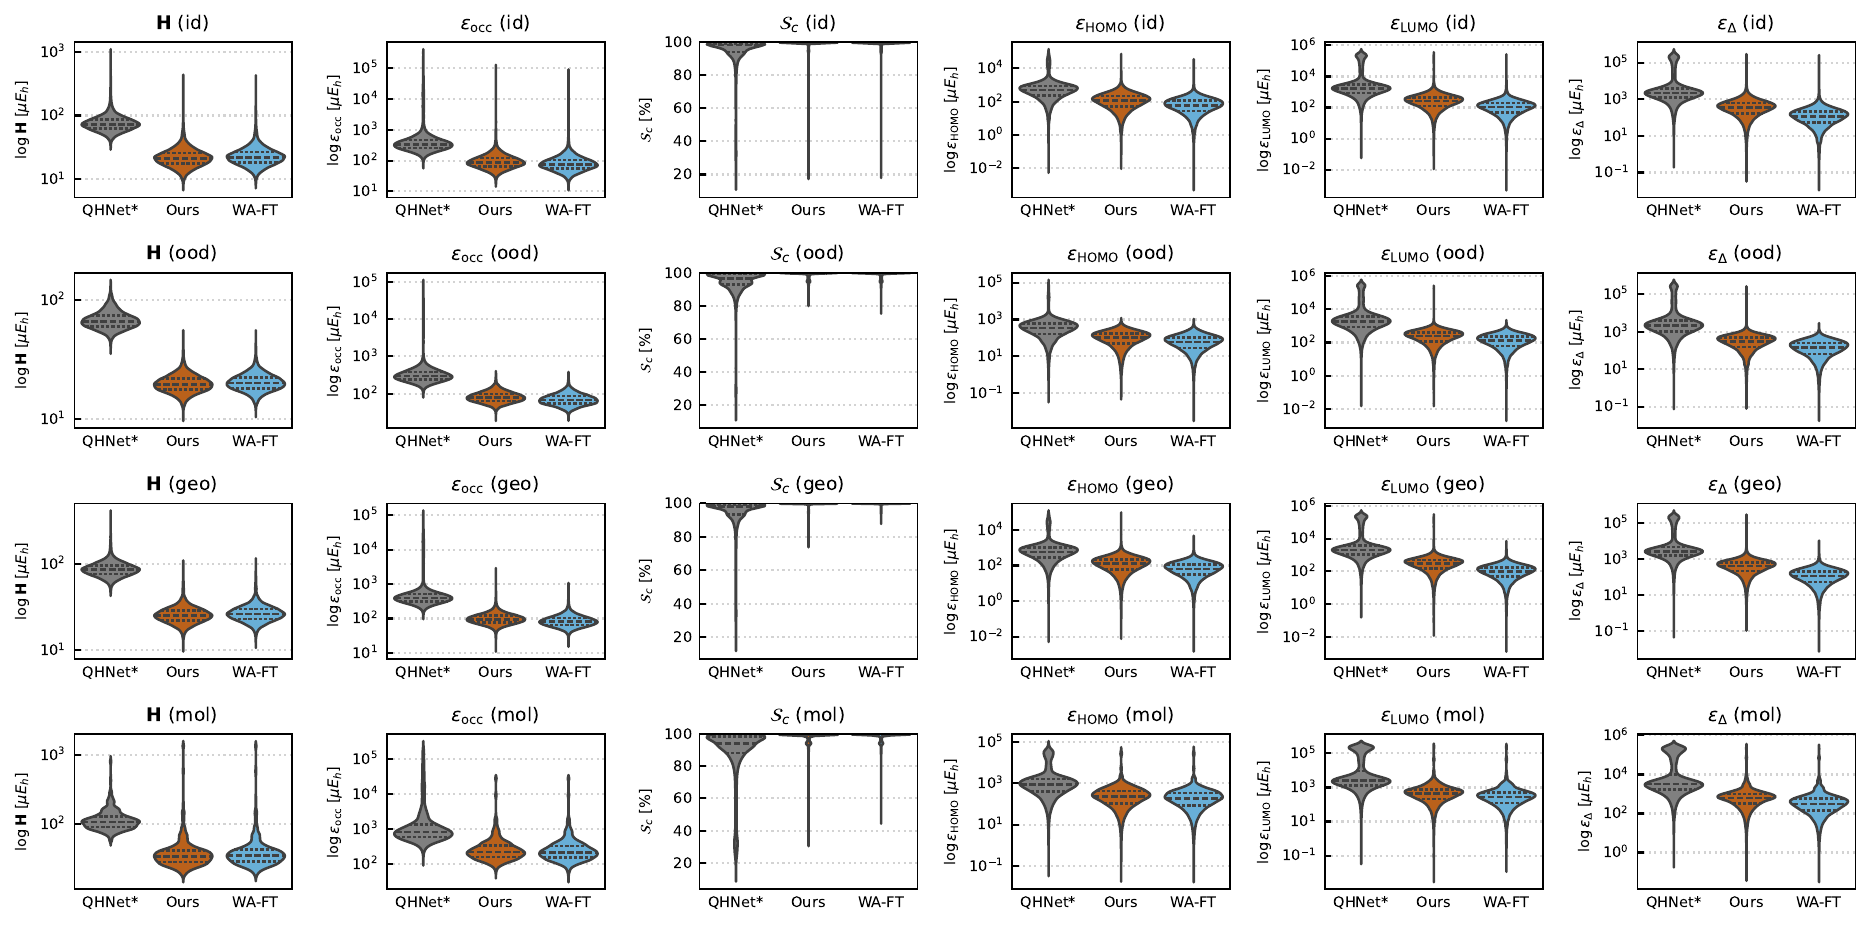}
    \caption{Violin plots compare QHNet* (gray), \QHFlow{}(orange), and its weighted-alignment fine-tune (WA-FT, cyan) on six metrics: Hamiltonian MAE ($\mathbf{H}$), occupied-orbital MAE ($\epsilon_{\text{occ}}$), \HOMO, \LUMO, \GAP ($\Delta$), and coefficient similarity (\SC).  Results are shown for the four evaluation splits — \texttt{id}, \texttt{ood}, \texttt{geo}, \texttt{mol}.  All axes are logarithmic except \SC.  Thick dashed lines mark the median; thin dashed lines indicate the quartiles.  Across every split the \QHFlow violins are both lower and narrower than those of QHNet*, and WA-FT delivers an additional (though smaller) improvement on the energy-related metrics.}
    \label{fig:prop_violin}
\end{figure}



%--- 첫 번째 서브 그림 ---------------------------------
\begin{figure}[t]   % 폭 조절: 0.5보다 조금 작게→여백 확보
    \centering
    \includegraphics[width=\linewidth]{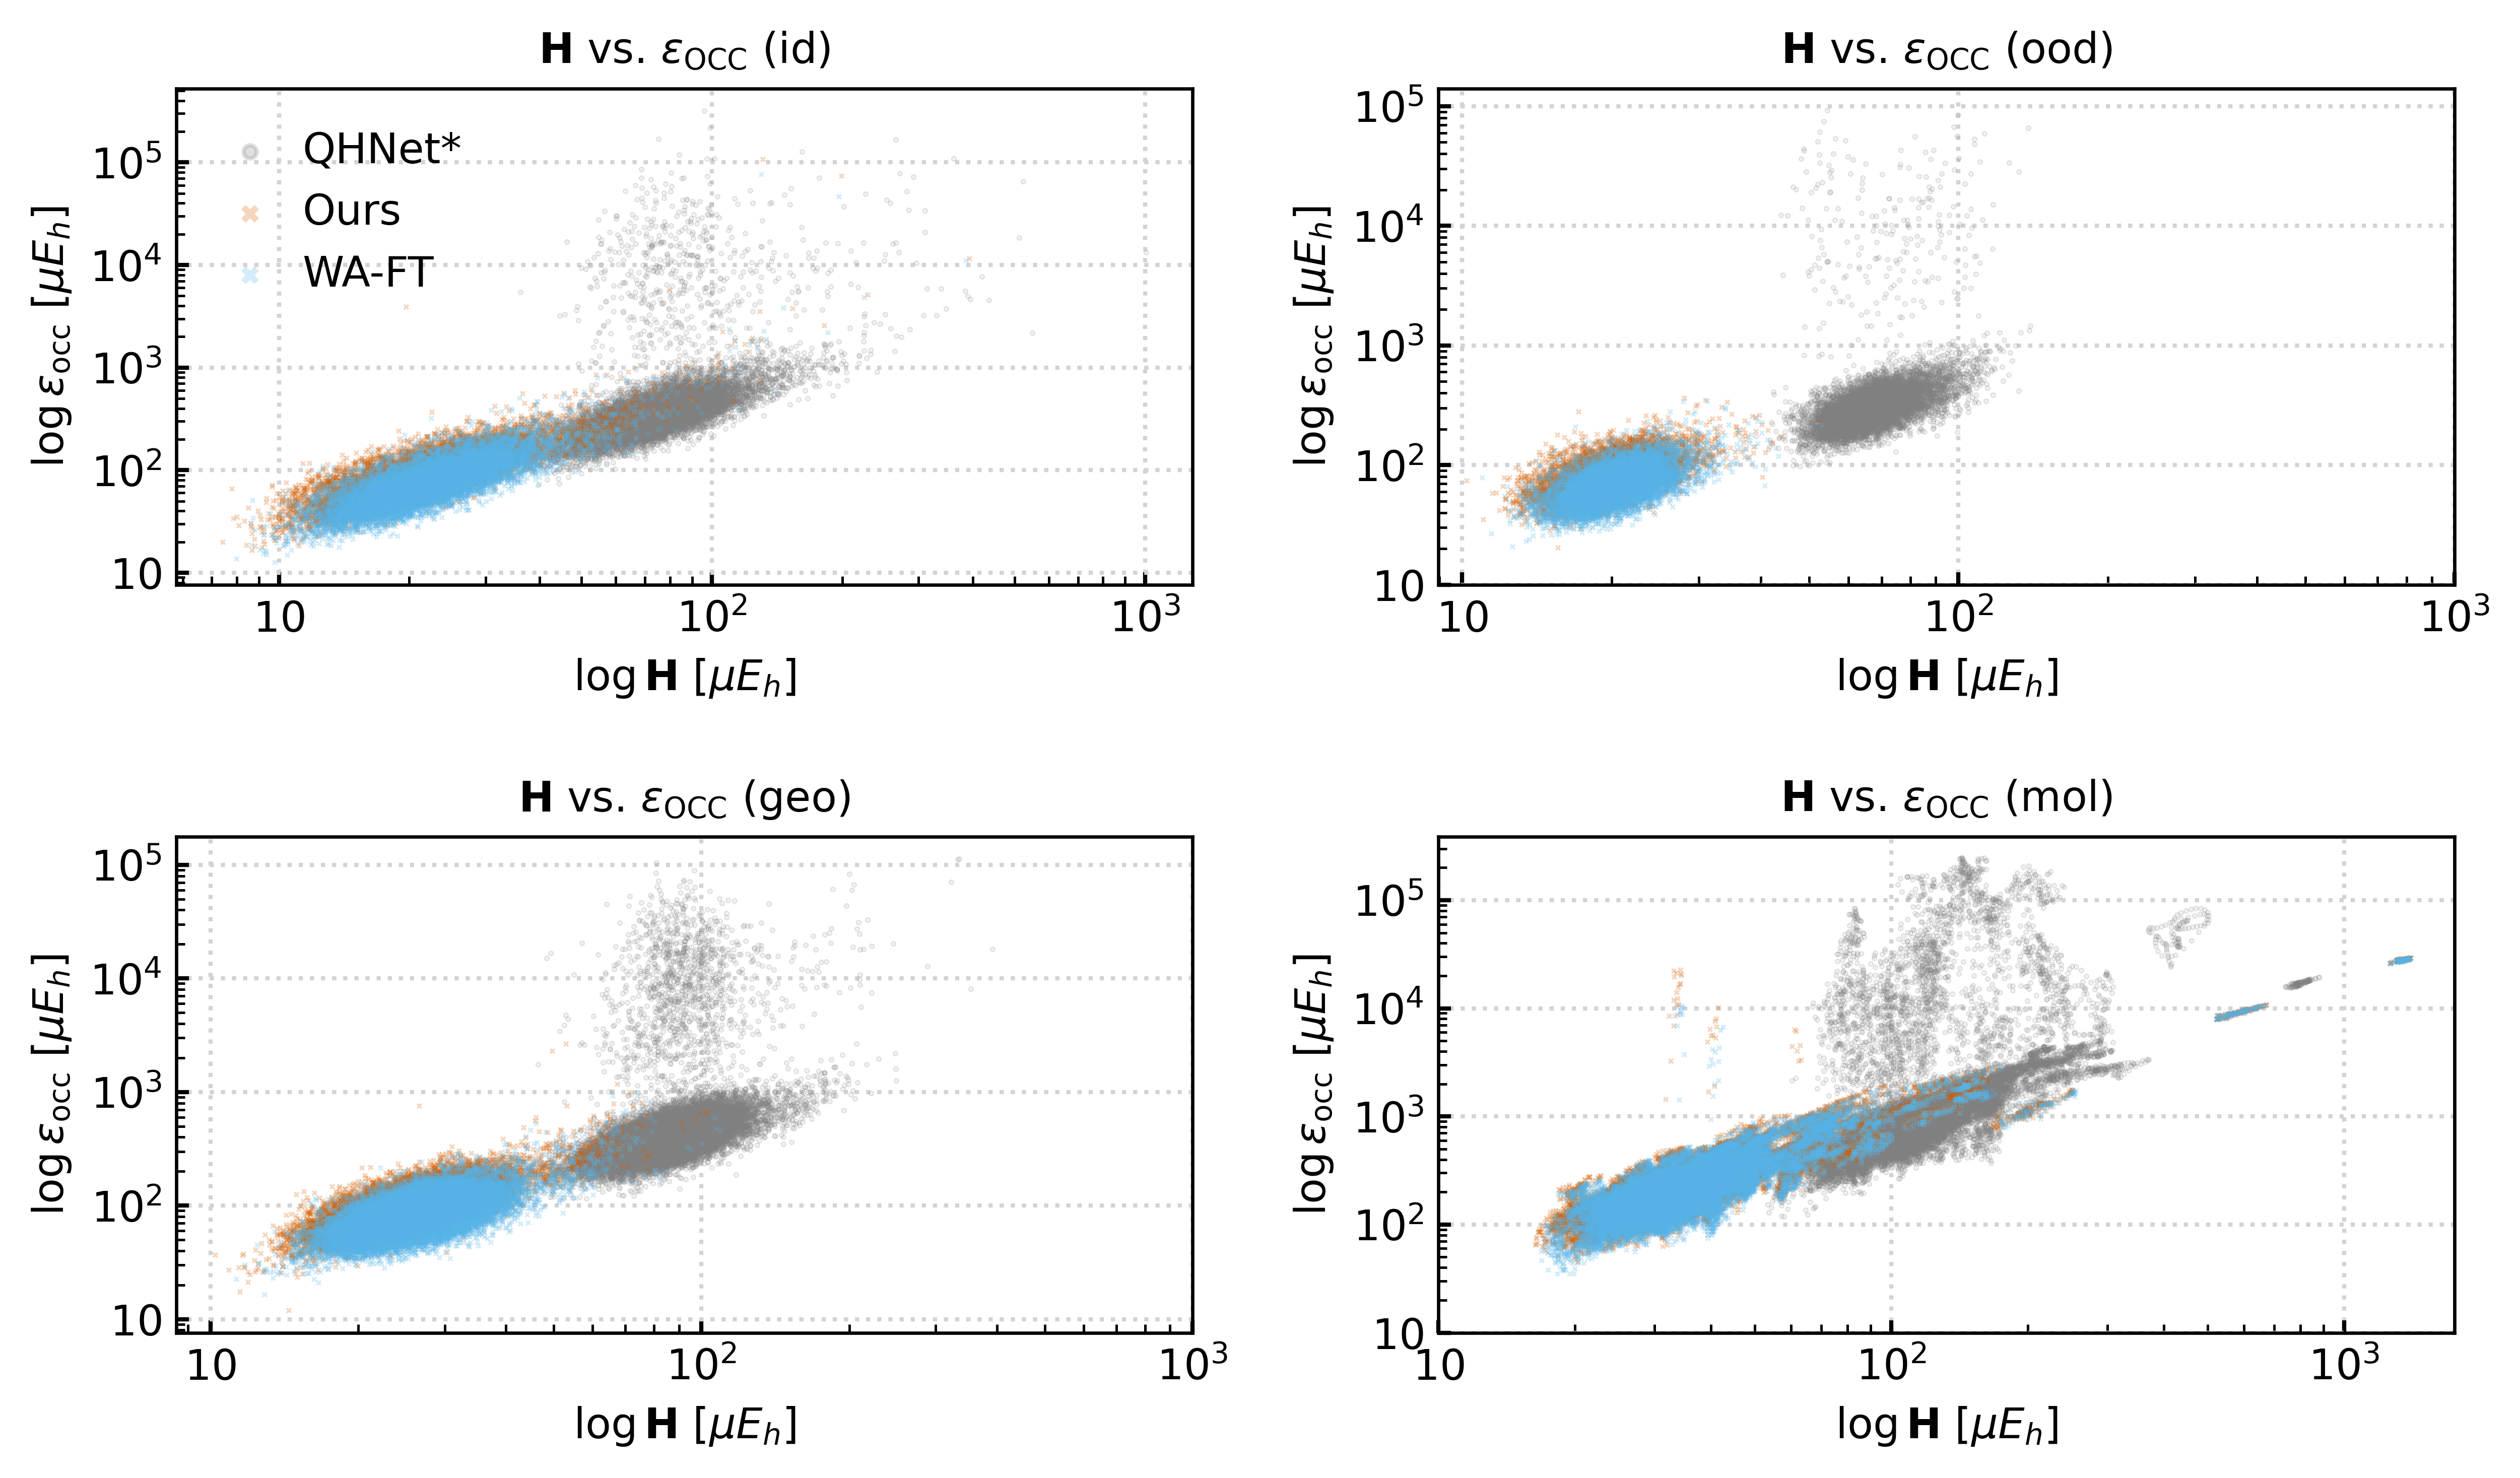}  % 그림 파일
    \caption{Scatter plots of $\log \mathbf{H}$ versus $\log\epsilon_{\text{occ}}$ for each QH9 split.  Points for QHNet* (gray) extend to the upper right, revealing frequent large joint errors.  \QHFlow{} (orange) and WA-FT (cyan) cluster tightly in the lower-left region, indicating that the flow-matching model achieves simultaneously low Hamiltonian and occupied-orbital errors, even on the challenging \texttt{ood} and \texttt{mol} splits.}                         % 서브캡션
    \label{fig:HvE}
\end{figure}% 서브 그림 사이 수평 여백
%--- 두 번째 서브 그림 ---------------------------------
\begin{figure}[t]
    \centering
    \includegraphics[width=\linewidth]{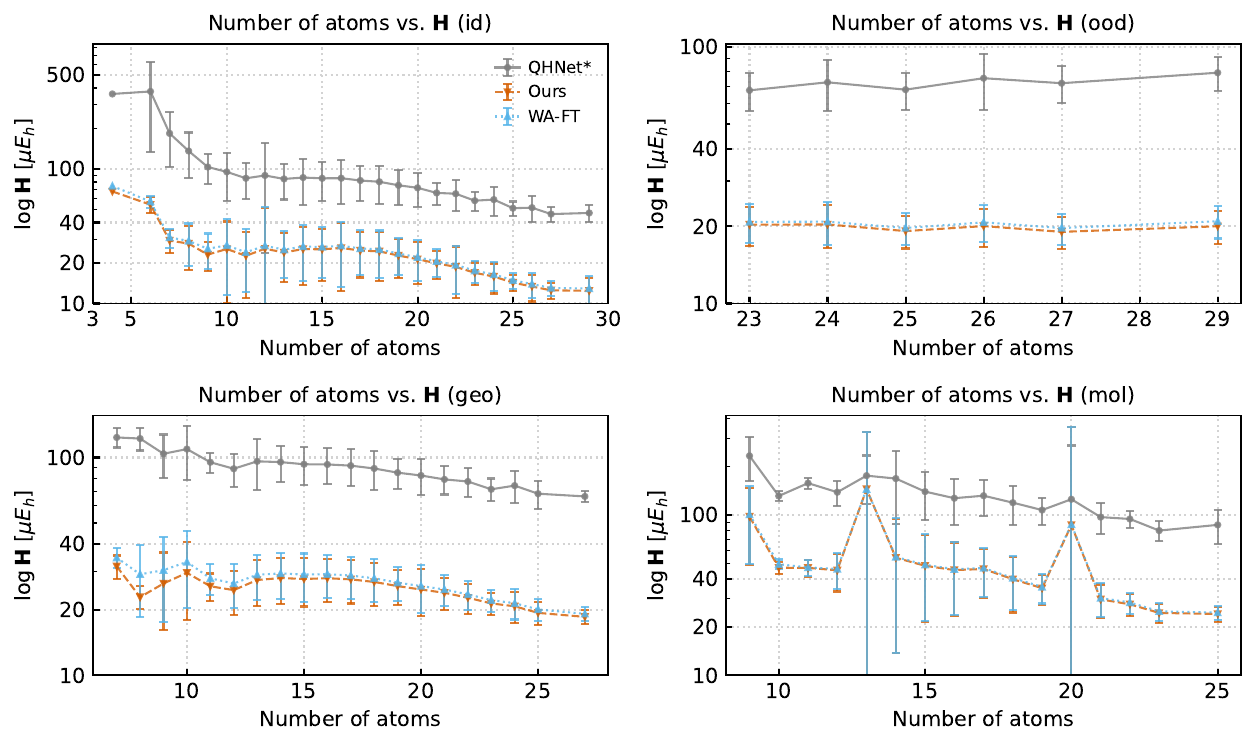}
    \caption{Mean log Hamiltonian error (markers) and one-standard-deviation bands (vertical bars) versus atom count for the four QH9 splits.  QHNet* (gray) errors rise with molecular size in \texttt{ood}, whereas \QHFlow{} (orange) and WA-FT (cyan) remain nearly flat up to 29 atoms. This suggests that modelling the full Hamiltonian distribution with symmetry-aware priors confers robust transferability to larger, more complex molecules.}
    \label{fig:NvH}
\end{figure}
%-------------------------------------------------------

% \subsection{Limitations}
% Our study demonstrates flow matching only on top of QHNet, mainly because its code is publicly available and its training cost is moderate. Although the approach should, in principle, be compatible with other SE(3) equivariant backbones (e.g., WANet or SPHNet), those implementations are not open-sourced, so we could not verify the transferability of our gains. Furthermore, the flow formulation increases the training time by approximately 10–20\% compared to the vanilla QHNet, due to the need to process intermediate Hamiltonians. Finally, all experiments are limited to gas-phase molecules of up to 29 atoms and to two common XC functionals (PBE and B3LYP). Extending the method to much larger systems, periodic solids, or higher-accuracy levels of theory (e.g., hybrid or double-hybrid functionals) is left for future work.

% \newpage
% \section*{Reproducibility Statement}

% We are committed to ensuring the reproducibility of our results. The codebase for QHFlow, including model implementations, training scripts, and evaluation protocols, will be made publicly available upon publication. We provide detailed descriptions of our model architecture, training objectives, hyperparameters, datasets, and experimental setups in the main text and Appendix. All datasets used in this work, including MD17 and QH9, are publicly accessible. Instructions for reproducing the training and evaluation results are included in the code repository.

% \section*{Ethics Statement}

% This work focuses on advancing machine learning methods for quantum chemistry applications and does not involve human subjects, personal data, or sensitive information. As such, we believe there are no direct ethical concerns associated with this research. Nevertheless, we acknowledge that improved computational tools for molecular modeling could have downstream applications in sensitive areas such as pharmaceuticals or materials development. We encourage responsible and ethical use of our methods in accordance with applicable laws and scientific guidelines.

% \subsection{SCF time.}
% \input{table/qh9_scf_time}

% \section{Additional related works}

% \textbf{SE(3) equivariant neural network.}
% SE(3)-equivariant neural networks~\cite{thomas2018tensor,brandstetter2021geometric,fuchs2020se,passaro2023reducing,luoenabling} have become foundational in machine learning applications for physics~\cite{batzner20223}, chemistry~\cite{kim2024mofflow}, and materials science~\cite{xie2021crystal,miller2024flowmm}, as they can naturally and efficiently handle the roto-translational symmetries inherent in molecular systems. These models have shown great performance in tasks such as learning interatomic potentials, predicting molecular forces~\cite{batatia2022mace,liao2022equiformer,liao2023equiformerv2}, and modeling charge densities~\cite{cheng2023equivariant,kim2024gaussian,fu2024recipe,koker2024higher}, offering accuracy and efficiency benefits. However, Hamiltonian matrices present a more challenging prediction target than scalar or vector quantities. Since Hamiltonians are matrix-valued and constructed in spherical harmonic bases, they must satisfy higher-order SO(3) equivariance, governed by Wigner D-representations~\cite{arfken2011mathematical,griffiths2018introduction}. This introduces unique modeling challenges and motivates the development of more expressive equivariant architectures that can handle symmetry-constrained outputs~\cite{unke2021se,yu2023efficient}.
